# Supplementary material for: Adaptive Estimation for Non-stationary Factor Models And A Test for Static Factor Loadings
Source: arXiv:2012.14708 source file (2024-02-03)
Supplement: Supplementary file 1 [file supplement.pdf]

# Supplemental Material for “Adaptive Estimation for Non-stationary Factor Models And A Test for Static Factor Loadings

Weichi Wu \*

Tsinghua University

Zhou Zhou †

University of Toronto

December 29, 2020

## Abstract

Section 1 of this supplementary material provides detailed assumptions for the evolutionary factor models, and a discussion of the rate in Theorem ?? of the main article. Section 2 gives out assumptions of and comments on Theorem ?? for the test of static factor loadings. Section 3 is regarding the power performance of the test of the static factor loading. Section 4 gives out the method for selecting tuning parameters. Section 5 contains the proofs of Theorem ??, ??, ?? for estimation of the null space of the evolutionary loading matrix. Section 6 includes the proof of Propositions ?? , ?? and Theorems ??, ?? for testing the static factor loading. Finally, Section 7 proves Theorem C.1.

## 1 Assumptions for the time-varying loading matrix

In this section we shall state our assumptions on the moment and dependency of the processes  $\mathbf{X}_i$ ,  $\mathbf{z}_i$  and  $\mathbf{e}_i$ . For this purpose we define further some notation. At time  $i/n$ , the  $d(i/n)$  dimensional factors  $\mathbf{z}_{i,n} = (z_{i,l_1,n}, \dots, z_{i,l_{d(i/n)},n})^\top$  where the index set  $\{l_1, \dots, l_{d(i/n)}\} \subset \{1, 2, \dots, d\}$ . Let  $\underline{\mathbf{Q}}(t, \mathcal{F}_i) = (Q_{l_1}(t, \mathcal{F}_i), \dots, Q_{l_{d(i/n)}}(t, \mathcal{F}_i))^\top$ . Denoted by  $\Sigma_z(t, k) = \mathbb{E}(\underline{\mathbf{Q}}(t, \mathcal{F}_{i+k})\underline{\mathbf{Q}}^\top(t, \mathcal{F}_i))$ ,  $\Sigma_e(t, k) = \mathbb{E}(\mathbf{H}(t, \mathcal{F}_{i+k})\mathbf{H}^\top(t, \mathcal{F}_i))$  the  $k_{th}$  order auto-covariance function of  $z_{i,n}$  and  $e_{i,n}$  at time  $t$ , respectively. Let  $\Sigma_{ze}(t, k) = \mathbb{E}(\underline{\mathbf{Q}}(t, \mathcal{F}_{i+k})\mathbf{H}^\top(t, \mathcal{F}_i))$ ,  $\Sigma_{ez}(t, k) = \mathbb{E}(\mathbf{H}(t, \mathcal{F}_{i+k})\underline{\mathbf{Q}}^\top(t, \mathcal{F}_i))$ . Let  $\mathcal{C}^K(\tilde{M})[0, 1]$  be the

---

\*The author gratefully acknowledges *NSFC Young program (No.11901337)*.

†The author gratefully acknowledges *NSERC*

collection of functions  $f$  defined on  $[0, 1]$  such that the  $K$ -th derivative of  $f$  is Lipschitz continuous with Lipschitz constant  $\tilde{M}$ . For  $\mathbf{F}$  matrix, let  $\|\mathbf{F}\|_2 = \sqrt{\lambda_{\max}(\mathbf{F}\mathbf{F}^\top)}$ . If  $\mathbf{F}$  is a vector, then  $\|\mathbf{F}\|_2 = \|\mathbf{F}\|_F$ . We first present assumptions on  $\mathbf{A}(t)$ .

(A1) Let  $a_{ij}(t)$ ,  $1 \leq i \leq p$ ,  $1 \leq j \leq d$  be the  $(i, j)_{th}$  element of  $\mathbf{A}(t)$ . We assume there exists a sufficiently large constant  $M$  such that

$$\sup_{t \in [0, 1]} |a_{ij}(t)| \leq M. \quad (\text{A.1})$$

(A2) Assume  $\sigma_{x,i,j}(t, k)$ ,  $1 \leq i \leq p$  and  $1 \leq j \leq p$ ,  $1 \leq k \leq k_0$  belongs to a common functional space  $\Omega$  which is equipped with an orthonormal basis  $B_j(t)$ , i.e.  $\int_0^1 B_m(t)B_n(t)dt = \mathbf{1}(m = n)$ , where  $\mathbf{1}(\cdot)$  is an indicator function. Assume  $\Omega \in \mathcal{C}^K(\tilde{M})[0, 1]$  for some  $K \geq 2$ . Moreover

$$\max_{1 \leq i \leq p, 1 \leq j \leq p} \sup_{t \in [0, 1]} |\sigma_{x,i,j}(t, k) - \sum_{u=1}^{J_n} \tilde{\sigma}_{x,i,j,u}(k) B_u(t)| = O_p(g_{J_n, K, \tilde{M}}), \quad (\text{A.2})$$

where  $\tilde{\sigma}_{x,i,j,u}(k) = \int_0^1 \sigma_{x,i,j}(t, k) B_u(t) dt$ , and  $g_{J_n, K, \tilde{M}} \rightarrow 0$  as  $J_n \rightarrow \infty$ .

Condition (A1) concerns the boundedness of the loading matrix, while (A2) means  $\Sigma_X(t, k)$  can be approximated by basis expansion. The approximation error rate  $g_{J_n, K, \tilde{M}}$  diminishes as  $J_n$  increases. Often higher differentiability yields more accurate approximation rate.

**Remark A.1.** Consider the case for  $1 \leq k \leq k_0$ ,  $1 \leq i, j \leq p$ ,  $\sigma_{x,i,j}^{(1)}(t, k), \dots, \sigma_{x,i,j}^{(v-1)}(t, k)$  are absolutely continuous in  $t$  where  $\sigma_{x,i,j}^{(m)}(t, k) = \frac{\partial^m \sigma_{x,i,j}(t, k)}{\partial t^m}$  for some positive integer  $m$ . We are able to specify the rate  $g_{J_n, m+1, \tilde{M}}$  for various basis functions.

(a) Assume i)  $\max_{1 \leq i, j \leq p, 1 \leq k \leq k_0} \int_0^1 \frac{\sigma_{x,i,j}^{(v+1)}(t)}{\sqrt{1-t^2}} dt \leq M < \infty$  for some constant  $M$ ,  $\sigma_{x,i,j}^{(v)}(t)$  is of bounded variation for all  $i, j$ , then the uniform approximation rate  $g_{J_n, m+1, \tilde{M}}$  is  $J_n^{-v+1/2}$  for normalized Legendre polynomial basis. If  $\sigma_{x,i,j}(t, k)$ 's are analytic inside and on a certain region in the complex plane then the approximation rate decays geometrically in  $J_n$ . See for instance Wang and Xiang (2012) for more details.

(b) If  $\sigma_{x,i,j}^{(v)}(t, k)$  is Lipschitz continuous, then the uniform approximation rate  $g_{J_n, m+1, \tilde{M}}$  is  $J_n^{-v}$  when trigonometric polynomials (if all  $\sigma_{x,i,j}(t, k)$  can be extended to periodic functions) or

orthogonal wavelets generated by sufficiently high order father and mother wavelets are used. See Chen (2007) for more details.

The assumptions for  $\mathbf{z}_{i,n}$  and  $\mathbf{e}_{i,n}$  are now in order.

(M1) The short-range dependence conditions hold for both  $\mathbf{z}_{i,n}$  and  $\mathbf{e}_{i,n}$  in  $\mathcal{L}^l$  norm, i.e.

$$\Delta_{Q,l,m} := \max_{1 \leq j \leq d} \sum_{k=m}^{\infty} \delta_{Q,l,j}(k) = o(1), \quad \Delta_{H,l,m} := \max_{1 \leq j \leq p} \sum_{k=m}^{\infty} \delta_{H,l,j}(k) = o(1) \quad (\text{A.3})$$

as  $m \rightarrow \infty$  for some constant  $l \geq 4$ .

(M2) There exists a constant  $M$  such that

$$\sup_{t \in [0,1]} \max_{1 \leq u \leq d} \mathbb{E}|Q_u(t, \mathcal{F}_0)|^4 \leq M, \quad \sup_{t \in [0,1]} \max_{1 \leq v \leq p} \mathbb{E}|H_v(t, \mathcal{F}_0)|^4 \leq M.$$

(M3) For  $t, s \in [0, 1]$ , there exists a constant  $M$  such that

$$(\mathbb{E}|Q_u(t, \mathcal{F}_0) - Q_u(s, \mathcal{F}_0)|^2)^{1/2} \leq M|t - s|, \quad 1 \leq u \leq d, \quad (\text{A.4})$$

$$(\mathbb{E}|H_v(t, \mathcal{F}_0) - H_v(s, \mathcal{F}_0)|^2)^{1/2} \leq M|t - s|, \quad 1 \leq v \leq p, \quad (\text{A.5})$$

$$(\mathbb{E}|G_v(t, \mathcal{F}_0) - G_v(s, \mathcal{F}_0)|^2)^{1/2} \leq M|t - s|, \quad 1 \leq v \leq p. \quad (\text{A.6})$$

Conditions (M1)-(M3) means that each coordinate process of  $\mathbf{z}_{i,n}$  and  $\mathbf{e}_{i,n}$  are standard short memory locally stationary time series defined in the literature; see for instance Zhou and Wu (2009). Furthermore, the moment condition (M2) implies that for  $0 \leq t \leq 1$ , all elements of the matrices  $\Sigma_{z,e}(t, k)$  and  $\Sigma_e(t, k)$  are bounded in  $\mathcal{L}^4$  norm.

We then postulate the following assumptions on the covariance matrices of the common factors  $\mathbf{z}_{i,n}$  and the idiosyncratic components  $\mathbf{e}_{i,n}$ , which are needed for spectral decomposition:

(S1) For  $t \in [0, 1]$  and  $k = 1, \dots, k_0$ , all components of  $\Sigma_e(t, k)$  are 0.

(S2) For  $k = 0, 1, \dots, k_0$ ,  $\Sigma_z(t, k)$  is full ranked on a sub-interval of  $[0, 1]$ .

(S3) For  $t \in [0, 1]$  and  $k = 1, \dots, k_0$ , all components of  $\Sigma_{ez}(t, k)$  are 0.

(S4) For  $t \in [0, 1]$  and  $1 \leq k \leq k_0$ ,  $\|\Sigma_{z,e}(t, k)\|_F = o(\eta_n^{1/2} p^{\frac{1-\delta}{2}})$ , where  $\eta_n$  is the sequence defined in condition (C1).

Condition (S1) indicates that  $\{\mathbf{e}_{i,n}\}$  does not have auto-covariance up to order  $k_0$  which is slightly weaker than the requirement that  $\{\mathbf{e}_{i,n}\}$  is a white noise process used in the literature. Condition (S2) implies that for  $1 \leq i \leq n$ , there exists a certain period that no linear combination of components of  $\mathbf{z}_{i,n}$  is white noise that can be absorbed into  $\mathbf{e}_{i,n}$ . (S3) implies that  $\mathbf{z}_{i,n}$ , and  $\{\mathbf{e}_{i+k,n}\}$  are uncorrelated for any  $k \geq 0$ . Condition (S4) requires a weak correlation between  $\mathbf{z}_{i+k}$  and  $\mathbf{e}_i$ . In fact it is the non-stationary extension of Condition (i) in Theorem 1 of Lam et al. (2011) and condition (C6) of Lam and Yao (2012). Though (C6) of Lam and Yao (2012) assumes a rate of  $o(p^{1-\delta})$ , it requires standardization of the factor loading matrix  $\mathbf{A}$ .

**Remark A.2.** We now discuss the equivalent assumptions on the fix dimensional loading matrix model (??). Define  $\Sigma_{z^*}(t, k)$ ,  $\Sigma_{z^*,e^*}(t, k)$ ,  $\Sigma_{e^*}(t, k)$ ,  $\Sigma_{e^*,z^*}(t, k)$  similarly to  $\Sigma_z(t, k)$ ,  $\Sigma_{z,e}(t, k)$ ,  $\Sigma_e(t, k)$ ,  $\Sigma_{e,z}(t, k)$  and assume (S) for these quantites. By construction conditions (M) are satisfied. In particular, under the equivalent model (A.4) and (A.5) imply (A.6). Conditions (A) are satisfied if each element of  $\mathbf{A}^*(t)$ ,  $\Sigma_{z^*}(t, k)$  and  $\Sigma_{z^*,e^*}(t, k)$ ,  $k = 0, \dots, k_0$  has a bounded  $K$  order derivative. Condition (C1) is satisfied with  $\mathcal{T}_{\eta_n}$  the period when smallest nonzero  $\sigma_u$  exceeds  $\eta_n$ . If  $d(t)$  is piecewise constant with bounded number of change points, then  $|\mathcal{T}_{\eta_n}| \rightarrow 1$  as  $n \rightarrow \infty$  and  $\eta_n \rightarrow 0$ . If  $d(t) \equiv d$  we can assume that  $\mathcal{T}_{\eta_n} = [0, 1]$  for some sufficiently small positive  $\eta_n := \eta > 0$ .

## 1.1 Discussion of The Rate in Theorem ??

**Remark A.3.** If we assume that  $\sigma_{x,i,j}(t, k)$ 's are real analytic and normalized Legendre polynomials or trigonometric polynomials (when all  $\sigma_{x,i,j}(t, k)$  can be extended to periodic functions) are used as basis, then Theorem ?? will yield an approximation rate of  $\frac{p^{2-\delta} \log n}{\sqrt{n}}$ . For Theorem ?? the approximation rate of (i) is then  $\frac{p^\delta \log n}{\sqrt{n}}$  and of (ii) is  $p^{-1/2} + \frac{p^{\delta/2} \log n}{\sqrt{n}}$  by taking  $J_n = M \log n$  for some large constant  $M$ . Our rate achieves the rate of Lam et al. (2011) for stationary high dimensional time series except a factor of logarithm. For Theorem ?? when  $\eta_n \equiv \eta$  for some fixed constant  $\eta$ , the approximation rate is  $\frac{p^{2-\delta} \log n}{n^{1/2}}$  for (i),  $\frac{p^2 \log^2 n}{n}$  for (ii) and  $\frac{p^{2\delta} \log^2 n}{n}$  for (iv) by taking  $J_n = M \log n$  for some large constant  $M$ . These rates coincide that of Theorem 1 and Corollary 1 of Lam and Yao (2012) except a factor of logarithm. The above findings are consistent with the results in nonparametric sieve estimation for analytic functions where the uniform convergence

rates for the sieve estimators (when certain adaptive sieve bases are used for the estimation) are only inferior than the  $n^{-1/2}$  parametric rate by a factor of logarithm. We shall also point out that the sieve approximation rates will be adaptive to the smoothness and will be slower when  $\sigma_{x,i,j}(t, k)$ 's are less smooth in which case  $g_{J_n, K, \tilde{M}}$  converges to zero at an adaptive but slower rate as  $J_n$  increases.

## 1.2 The moment condition (M') for proposition ??

The following mild moment condition (M') is needed for proposition ??.

(M') There exists an integer  $l > 2$  and a universal constant  $M$  such that  $\max_{1 \leq j \leq d} \sum_{k=1}^{\infty} \delta_{Q, 2l, j}(k) < \infty$ ,  $\max_{1 \leq j \leq p} \sum_{k=1}^{\infty} \delta_{H, 2l, j}(k) < \infty$  and

$$\sup_{t \in [0, 1]} \max_{1 \leq u \leq d} \mathbb{E}|Q_u(t, \mathcal{F}_0)|^{2l} \leq M, \quad \sup_{t \in [0, 1]} \max_{1 \leq v \leq p} \mathbb{E}|H_v(t, \mathcal{F}_0)|^{2l} \leq M.$$

## 2 Assumptions of and comments on Theorem ??

(a)  $\|\mathbf{A}\|_{\infty} \lesssim 1$ .

(b)  $l \geq 4$ .

(c)  $(N_n p^2)^{1/l} \lesssim m_n^{\frac{3-25\zeta}{32}}$  and  $k_0 N_n(p-d)p \lesssim \exp(m_n^{\zeta})$  for some  $0 \leq \zeta < 1/11$ .

(d) Let  $\sigma_{j,j} = \sum_{i,l=1}^{m_n} \text{cov}(\tilde{Z}_{i,j}, \tilde{Z}_{l,j})/m_n$ . There exists  $\eta > 0$  such that  $\min \sigma_{j,j} \geq \eta$ , i.e., each of the  $k_0 N_n p(p-d)$  univariate sub-series of  $\tilde{\mathbf{Z}}_i$  is non-degenerated.

(e) The dependence measure for  $\mathbf{X}_{i,n}$  satisfies

$$\delta_{G, 2l}(k) = O(((k+1) \log(k+1))^{-2}). \quad (\text{B.7})$$

(f) There exists a constant  $M_{2l}$  depending on  $l$  such that for  $1 \leq i \leq n$ , and for all  $p$  dimensional vector  $\mathbf{c}$  such that  $\|\mathbf{c}\|_2 = 1$ , the inequality  $\|\mathbf{c}^{\top} \mathbf{e}_{i,n}\|_{\mathcal{L}^{2l}} \leq M_{2l} \|\mathbf{c}^{\top} \mathbf{e}_{i,n}\|_{\mathcal{L}^2}$  holds. Also  $\max_{1 \leq i \leq n} \lambda_{\max}(\text{cov}(\mathbf{e}_{i,n} \mathbf{e}_{i,n}^{\top}))$  is uniformly bounded as  $n$  and  $p$  diverges.

The rate of Theorem ?? is defined by

$$\begin{aligned} \iota(n, p, q, D_n) = \min & (n^{-1/8} M^{1/2} l_n^{7/8} + \gamma + (n^{1/8} M^{-1/2} l_n^{-3/8})^{q/(1+q)} (\sum_{j=1}^p \Theta_{M,j,q}^q)^{1/(1+q)} \\ & + \Xi_M^{1/3} (1 \vee \log(p/\Xi_M))^{2/3}), \end{aligned} \quad (\text{B.8})$$

where the minimum is taken over all possible values of  $\gamma$  and  $M$  subject to  $n^{3/8} M^{-1/2} l_n^{-5/8} \geq \max\{D_n(n/\gamma)^{1/4}, l_n^{1/2}\}$ . Here  $l_n = \log(pn/\gamma) \vee 1$ ,  $\Theta_{M,j,q} = \sum_{k=M}^{\infty} \delta_{G,q,j}(k)$  and  $\Xi_M = \max_{1 \leq j \leq p} \sum_{k=M}^{\infty} k \delta_{G,2,j}(k)$ .

Conditions (a)-(e) control the magnitude of the loading matrix, the dimension and dependence of the time series  $\mathbf{X}_{i,n}$  as well as non-degeneracy of the process  $\tilde{\mathbf{Z}}_i$ . Those conditions are standard in the literature of high dimensional Gaussian approximation; see for instance Zhang and Cheng (2018). Condition (f) controls the magnitude of the  $\mathcal{L}^{2l}$  norm of projections of  $\mathbf{e}_{i,n}$  by their  $\mathcal{L}^2$  norm which essentially requires that the dependence among the components of  $\mathbf{e}_{i,n}$  cannot be too strong. (f) is mild in general and is satisfied, for instance, if the components of  $\mathbf{e}_{i,n}$  are independent or  $\mathbf{e}_{i,n}$  is a sub-Gaussian random vector with a variance proxy that does not depend on  $p$  for each  $i$ . Furthermore, we comment that Condition (d) is a mild non-degeneracy condition. For example, assuming (i)  $\mathbf{e}_{s,n}$  is independent of  $\mathbf{e}_{l,n}$ ,  $\mathbf{z}_{l,n}$  for  $s \geq l$ ,  $\min_{1 \leq i \leq n, 1 \leq j \leq p} \mathbb{E} X_{i,j}^2 \geq \eta' > 0$ ,  $\min_{1 \leq i \leq n} \lambda_{\min}(\text{cov}(\mathbf{e}_{i,n} \mathbf{e}_{i,n}^\top)) \geq \eta'' > 0$  for some constants  $\eta'$  and  $\eta''$ , and (ii) condition (a)-(c), (e) and (f) hold, then condition (d) holds. To see this, note that under null hypothesis, for  $1 \leq s \leq p-d$ ,  $1 \leq k \leq k_0$ ,  $1 \leq i, j \leq n$  and  $1 \leq v \leq p$ , we have for  $i \neq j$ ,

$$\mathbb{E}(\mathbf{F}_s^\top \mathbf{X}_{i+k,n} X_{i,v} \mathbf{F}_s^\top \mathbf{X}_{l+k,n} X_{l,v}) = \mathbb{E}(\mathbf{F}_s^\top \mathbf{e}_{i+k,n} X_{i,v} \mathbf{F}_s^\top \mathbf{e}_{l+k,n} X_{l,v}) = 0, \quad (\text{B.9})$$

$$\mathbb{E}((\mathbf{F}_s^\top \mathbf{X}_{i+k,n} X_{i,v})^2) = \mathbb{E}((\mathbf{F}_s^\top \mathbf{e}_{i+k,n} X_{i,v})^2) = \mathbf{F}_s^\top (\text{cov}(\mathbf{e}_{i+k,n} \mathbf{e}_{i+k,n}^\top)) \mathbf{F}_s \mathbb{E}(X_{i,v}^2) \geq \eta' \eta''. \quad (\text{B.10})$$

Consequently (B.9) and (B.10) imply condition (d).

### 3 Power

In this section we discuss the local power of our bootstrap-assisted testing algorithm in Section ?? of the main article for testing static factor loadings. For two matrices  $\mathbf{A}$  and  $\mathbf{B}$ , denoted by  $\mathbf{A} \circ \mathbf{B}$  the Hadamard product of  $\mathbf{A}$  and  $\mathbf{B}$ . Let  $\mathbf{J}$  be a  $p \times d$  matrix with all entries 1 where  $d = \text{rank}(\mathbf{A})$ .

To simplify the proof, we further assume the following Condition (G):

(G1):  $\mathbf{e}_i$  is independent of  $\mathbf{z}_s, \mathbf{e}_s$  for  $i > s$ .

(G2): the dependence measure of  $\mathbf{z}_i$  satisfies

$$\max_{1 \leq j \leq d} \delta_{Q,4,j}(k) = O(((k+1) \log(k+1))^{-2}). \quad (\text{C.1})$$

(G3): the dependence measures of  $\mathbf{e}_i$  satisfy

$$\sum_{k=1}^{\infty} k \sup_{0 \leq t \leq 1} \|\mathbf{F}^\top \mathbf{H}(t, \mathcal{F}_i) - \mathbf{F}^\top \mathbf{H}(t, \mathcal{F}_i^{(i-k)})\|_{\mathcal{L}^4} = O(\log^2 p) \quad (\text{C.2})$$

for all  $p$  dimensional vector  $\mathbf{F}$  such that  $\|\mathbf{F}\|_F = 1$ .

Conditions (G1) are (G2) and mild further assumptions on the error and factor processes. Condition (G3) controls the strength of temporal dependence for projections of the error process  $\mathbf{e}_i$ . (G3) essentially requires that each component of  $\mathbf{e}_i$  is a short memory process and the dependence among the components of  $\mathbf{e}_i$  are not too strong. Elementary calculation shows that Condition (G3) is satisfied under two important scenarios. The first is that the dependence measures satisfy  $\max_{1 \leq j \leq p} \delta_{H,4,j}(k) = O(\chi^k)$  for some  $\chi \in (0, 1)$ . See Lemma C.1. The second is that each component of process  $\mathbf{e}_i$  are independent i.e.,  $H_{j_1}(\cdot, \mathcal{F}_u)$  is independent of  $H_{j_2}(\cdot, \mathcal{F}_v)$  for all  $u, v \in \mathbb{N}$  as long as  $j_1 \neq j_2$ ,  $1 \leq j_1, j_2 \leq p$ , and  $\sum_{k=1}^{\infty} k \max_{1 \leq j \leq p} \delta_{H,4,j}(k) = O(1)$ .

**Lemma C.1.** *Under conditions (f), (M') and  $\max_{1 \leq j \leq p} \delta_{H,4,j}(k) = O(\chi^k)$  for some  $\chi \in (0, 1)$ , (G3) holds.*

*Proof.* Notice that by condition (f), there exist constants  $M_1$  and  $M_2$  such that

$$\|\mathbf{F}^\top \mathbf{H}(t, \mathcal{F}_i) - \mathbf{F}^\top \mathbf{H}(t, \mathcal{F}_i^{(i-k)})\|_{\mathcal{L}^4} \leq 2\|\mathbf{F}^\top \mathbf{H}(t, \mathcal{F}_i)\|_{\mathcal{L}^4} \leq M_1 \|\mathbf{F}^\top \mathbf{H}(t, \mathcal{F}_i)\|_{\mathcal{L}^4} \leq M_2. \quad (\text{C.3})$$

On the other hand, by triangle inequality

$$\|\mathbf{F}^\top \mathbf{H}(t, \mathcal{F}_i) - \mathbf{F}^\top \mathbf{H}(t, \mathcal{F}_i^{(i-k)})\|_{\mathcal{L}^4} \leq \sum_{j=1}^p F_j \|H_j(t, \mathcal{F}_i) - H_j(t, \mathcal{F}_i^{(i-k)})\|_{\mathcal{L}^4} = O(\sqrt{p}\chi^k), \quad (\text{C.4})$$

where the last equality is due to Cauchy-Schwarz inequality and Condition (M'). As a consequence, (C.3) and (C.4) lead to that

$$\sup_{0 \leq t \leq 1} \|\mathbf{F}^\top \mathbf{H}(t, \mathcal{F}_i) - \mathbf{F}^\top \mathbf{H}(t, \mathcal{F}_i^{(i-k)})\|_{\mathcal{L}^4} = O(1 \wedge \sqrt{p} \chi^k). \quad (\text{C.5})$$

Notice that when  $k = \lfloor a \log p \rfloor$  for some sufficiently large constant  $a$ ,  $\sqrt{p} \chi^k = O(1)$ . Therefore by (C.5),

$$\begin{aligned} \sum_{k=1}^{\lfloor a \log p \rfloor} k \sup_{0 \leq t \leq 1} \|\mathbf{F}^\top \mathbf{H}(t, \mathcal{F}_i) - \mathbf{F}^\top \mathbf{H}(t, \mathcal{F}_i^{(i-k)})\|_{\mathcal{L}^4} + \sum_{k=\lfloor a \log p \rfloor + 1}^{\infty} k \sup_{0 \leq t \leq 1} \|\mathbf{F}^\top \mathbf{H}(t, \mathcal{F}_i) - \mathbf{F}^\top \mathbf{H}(t, \mathcal{F}_i^{(i-k)})\|_{\mathcal{L}^4} \\ = O(\log^2 p) + O\left(\sum_{k=\lfloor a \log p \rfloor + 1}^{\infty} k \chi^k\right) = O(\log^2 p), \end{aligned}$$

which finishes the proof.  $\square$

We consider the following class of local alternatives:

$$H_A : \mathbf{A}(t) = \mathbf{A}_n(t) := \mathbf{A} \circ (\mathbf{J} + \rho_n \mathbf{D}(t)), \quad (\text{C.6})$$

where  $\mathbf{D}(t) = (d_{ij}(t))$  is a  $p \times d$  matrix,  $\max_{i,j} \sup_t |d_{ij}(t)| \lesssim 1$ ,  $\sup_{t \in [0,1]} \|\mathbf{D}(t) \circ \mathbf{A}(t)\|_F = O(p^{\frac{1-\delta_1}{2}})$  for some  $\delta_1 \in [\delta, 1]$  and  $\rho_n \downarrow 0$  controls the magnitude of deviation from the null. Notice that, under the alternative hypothesis,  $\mathbf{A}_n(t)$  is a function of  $\rho_n$  and therefore

$$\int_0^1 \Sigma_X(t, k) dt = \int_0^1 \mathbf{A}_n(t) (\Sigma_z(t, k) \mathbf{A}_n(t)^\top + \Sigma_{z,e}(t, k)) dt := \gamma(\rho_n, k), \quad k > 0.$$

Let  $\mathbf{\Gamma}_k(\rho_n) = \gamma(\rho_n, k) \gamma(\rho_n, k)^\top$  and  $\mathbf{\Gamma}(\rho_n) = \sum_{k=1}^{k_0} \mathbf{\Gamma}_k(\rho_n)$ . To simplify notation, write  $\mathbf{\Gamma}(\rho_n)$ ,  $\rho_n > 0$  as  $\mathbf{\Gamma}_n$  with an orthogonal basis  $\mathbf{F}_n = (\mathbf{F}_{1,n}, \dots, \mathbf{F}_{p-d,n})$ . Recall the centered  $k_0 N_n(p-d)p$  dimensional Gaussian random vectors  $\mathbf{Y}$  and  $\mathbf{Y}_i$  defined in Theorem ?? of the main article and the definition of  $\tilde{\mathbf{Z}}_i$ . Define  $\tilde{\mathbf{Z}}_i$  in analogue of  $\tilde{\mathbf{Z}}_i$  with  $\mathbf{F}$  replaced by  $\mathbf{F}_n$ .

**Theorem C.1.** *Consider the alternative hypothesis (C.6). Assume in addition that for  $t \in [0, 1]$ ,  $\text{rank}(A(t)) = d$ ,  $p^\delta n^{-1/2} m_n^{1/2} \Omega_n = o(1)$ , and  $\Delta_n = |\sum_{i=1}^{m_n} \mathbb{E} \tilde{\mathbf{Z}}_i / m_n|_\infty \asymp \rho_n p^{\frac{1-\delta_1}{2}}$ . Then under conditions of Theorem ?? and condition (G) we have the following results.*

(a) Under the considered alternative hypothesis, if  $\rho_n m_n^{1/2} \log^{1/2} n \Omega_n = o(1)$  then

$$\begin{aligned} & \sup_{t \in \mathbb{R}} |\mathbb{P}(\hat{T}_n \leq t) - \mathbb{P}(|\mathbf{Y}|_\infty \leq t)| \\ &= O \left( \left( (\rho_n p^{\frac{\delta - \delta_1}{2}} + \frac{p^\delta}{\sqrt{n}}) \sqrt{m_n \log n \Omega_n} \right)^{1/3} + \left( \rho_n \sqrt{m_n \log n \Omega_n} \right)^{1/2} \right. \\ & \quad \left. + \iota(m_n, k_0 N_n p(p-d), 2l, (N_n p^2)^{1/l}) \right), \end{aligned} \quad (\text{C.7})$$

where the function  $\iota$  is defined in (B.8). Furthermore, if  $\sqrt{m_n} \rho_n p^{\frac{1-\delta_1}{2}} \rightarrow \infty$  then  $\hat{T}_n$  diverges at the rate of  $\sqrt{m_n} \rho_n p^{\frac{1-\delta_1}{2}}$ .

(b) Assume in addition the conditions of Theorem ?? hold, then if  $\Theta_n^{1/3} \log^{2/3}(\frac{W_{n,p}}{\Theta_n}) = o(1)$ ,

$$\begin{aligned} & \sup_{t \in \mathbb{R}} |\mathbb{P}(|\mathbf{Y}|_\infty \leq t) - \mathbb{P}(|\boldsymbol{\kappa}_n|_\infty \leq t | \mathbf{X}_i, 1 \leq i \leq n)| \\ &= O_p \left( \Theta_n^{1/3} \log^{2/3} \left( \frac{W_{n,p}}{\Theta_n} \right) + \left( \left( \frac{p^\delta}{\sqrt{n}} + \rho_n \right) \sqrt{w_n \Omega_n} \right)^{l/(1+l)} \right). \end{aligned} \quad (\text{C.8})$$

Furthermore,  $|\boldsymbol{\kappa}_n|_\infty = O_p(\sqrt{w_n} \rho_n p^{\frac{1-\delta_1}{2}} \sqrt{\log n})$ .

Therefore by (a) and (b) if  $\frac{\sqrt{m_n}}{\sqrt{w_n \log n}} \rightarrow \infty$ ,  $\sqrt{m_n} \rho_n p^{\frac{1-\delta_1}{2}} \rightarrow \infty$ , the power of the test approaches 1 as  $n \rightarrow \infty$ .

We introduce  $\delta_1$  to allow that  $\mathbf{D}(t)$  has a different level of strength than that of  $\mathbf{A}$ . For instance, if  $\mathbf{D}(t)$  has a bounded number of non-zero entries, then  $\delta_1 = 1$  while  $\delta$  can be any number in  $[0, 1]$ . The condition that  $\Delta_n \asymp \rho_n p^{\frac{1-\delta_1}{2}}$  is mild. In fact, it is shown in equation (G.8) in the proof of Proposition G.2 that  $|\mathbb{E} \tilde{\mathbf{Z}}_i|_\infty = O(\rho_n p^{\frac{1-\delta_1}{2}})$ , which means  $\Delta_n = O(\rho_n p^{\frac{1-\delta_1}{2}})$ . On the other hand, the condition  $\Delta_n \asymp \rho_n p^{\frac{1-\delta_1}{2}}$  requires that there exists at least one eigenvector of the null space of  $\sum_{k=1}^{k_0} \mathbf{\Gamma}_k$  such that an order  $p$  of its entries have the same order of magnitude.

## 4 Selection of Tuning Parameters

### 4.1 Selection of tuning parameters for the estimation of time-varying factor loading matrices.

We discuss the selection of  $J_n$  for the estimation of time-varying factors. Since in practice  $\beta_n$  is unknown, a data-driven method to select  $J_n$  is desired. By Theorem ??, the residuals  $\hat{\mathbf{e}}_{i,n} = \mathbf{X}_{i,n} - \hat{\mathbf{V}}(\frac{i}{n})\hat{\mathbf{V}}^\top(\frac{i}{n})\mathbf{X}_{i,n}$ . Notice that  $\hat{\mathbf{e}}_{i,n} = (\hat{e}_{i,1,n}, \dots, \hat{e}_{i,p,n})^\top$  is a  $p$  dimensional vector. We select  $J_n$  as the minimizer of the following cross validation standard  $CV(d)$

$$CV(d) = \sum_{i=1}^n \sum_{s=1}^p \frac{\hat{e}_{i,s,n}^2(d)}{(1 - v_{i,s}(d))^2} \quad (\text{D.1})$$

where  $v_{i,s}(d)$  is the  $s$ th diagonal element of  $\hat{\mathbf{V}}(\frac{i}{n})\hat{\mathbf{V}}^\top(\frac{i}{n})$  obtained by setting  $J_n = d$ , and  $\hat{e}_{i,s,n}(d)$ 's  $1 \leq i \leq n$ ,  $1 \leq s \leq p$  are also the residuals calculated when  $J_n = d$ . The cross-validation has been widely used in the literature of sieve nonparametric estimation and has been advocated by for example Hansen (2014). We choose  $J_n = \text{argmin}_d(CV(d))$  in our empirical studies.

### 4.2 Selection of tuning parameters $m_n$ and $w_n$ for testing static factor loadings

We select  $m_n$  by first select  $N_n$  and let  $m_n = \lfloor (n - k_0)/N_n \rfloor$ . The  $N_n$  is chosen by the minimal volatility method as follows. For a given data set, let

$$\hat{T}(N_n) = \sqrt{m_n} \max_{1 \leq k \leq k_0} \max_{1 \leq j \leq N_n} \max_{1 \leq i \leq p - \hat{d}_n} |\hat{\mathbf{F}}_i^\top \hat{\Sigma}_X(j, k)|_\infty \quad (\text{D.2})$$

be the test statistic obtained by using the integer parameter  $N_n$  with  $\hat{d}_n = \text{argmin}_{1 \leq i \leq R} \lambda_{i+1}(\hat{\Gamma})/\lambda_i(\hat{\Gamma})$  where  $R$  is defined in (??) of the main article.

Consider a set of candidate  $N_n$ , which is denoted by  $J = \{J_1, \dots, J_s\}$  where  $J_s$  are positive integers. For each  $J_v$ ,  $1 \leq v \leq s$  we calculate  $\hat{T}(N_n)$  and hence the local standard error

$$SE(\hat{T}(J_l), h) = \left( \frac{1}{2h} \sum_{u=-h}^h \left( \hat{T}(J_{u+l}) - \frac{1}{2h+1} \sum_{u=-h}^h \hat{T}(J_{u+l}) \right)^2 \right)^{1/2} \quad (\text{D.3})$$

where  $1 + h \leq l \leq s - h$  and  $h$  is a positive integer, say  $h = 1$ . We then select  $N_n$  by

$$\underset{1+h \leq l \leq s-h}{\operatorname{argmin}} SE(\hat{T}(J_l, h)) \quad (\text{D.4})$$

which stabilizes the test statistics. The idea behind the minimum volatility method is that the test statistic should behave stably as a function of  $N_n$  when the latter parameter is in an appropriate range. In our empirical studies we find that the proposed method performs reasonably well, and the results are not sensitive to the choice of  $N_n$  ( $m_n$ ) as long as  $N_n$  ( $m_n$ ) used is not very different from that chosen by (D.4).

After choosing  $m_n$ , we then further choose  $w_n$  by the minimal volatility method. In this case we first obtain the  $k_0 N_n(p - d)p$  dimensional vectors  $\{\hat{\mathbf{Z}}_i, 1 \leq i \leq m_n\}$  defined in Section ?? of the main article. Then we select  $w_n$  by a multivariate extension of the minimal volatility method in Zhou (2013) as follows. We consider choosing  $w_n$  from a grid  $w_1 \leq \dots \leq w_r$ . For each  $w_n = w_i$ ,  $1 \leq i \leq r$  we calculate a  $k_0 N_n(p - d)p$  dimensional vector  $\mathbf{B}_{i,r}^o = \operatorname{Vec}(\frac{1}{w_i(m_n - w_i + 1)} \sum_{j=1}^r (\hat{\mathbf{S}}_{j,w_i} - \frac{w_i}{m_n} \hat{\mathbf{S}}_{m_n})^{\circ 2})$  where  $\circ$  represents the Hadamard product and  $1 \leq r \leq m_n - w_r + 1$ . Let  $\mathbf{B}_i^o = (\mathbf{B}_{i,1}^{o\top}, \dots, \mathbf{B}_{i,m_n - w_r + 1}^{o\top})^\top$  be a  $k_0 N_n(p - d)p(m_n - w_r + 1)$  dimensional vector, and  $\mathbf{B}$  be a  $k_0 N_n(p - d)p(m_n - w_r + 1) \times r$  matrix with its  $i_{th}$  column  $\mathbf{B}_i^o$ . Then for each row, say  $i_{th}$  row  $\mathbf{B}_{i,\cdot}$  of  $\mathbf{B}$ , we calculate  $SE(\mathbf{B}_{i,\cdot}, h)$  for a given window size  $h$ , see (D.3) for definition of  $SE$  and therefore obtain a  $r - 2h$  length row vector. Stacking these row vectors we get a new  $k_0 N_n(p - d)p(m_n - w_r + 1) \times (r - 2h)$  matrix  $\mathbf{B}^\dagger$ . Let  $\operatorname{colmax}(\mathbf{B}^\dagger)$  be a  $(r - 2h)$  length vector with its  $i_{th}$  element being the maximum entry of the  $i_{th}$  column of  $\mathbf{B}^\dagger$ . Then we choose  $w_n = w_k$  if the smallest entry of  $\operatorname{colmax}(\mathbf{B}^\dagger)$  is its  $(k - h)_{th}$  element.

## 5 Proofs of Theorem ??, ??, ?? and Proposition ??.

We now present some additional notation for the proofs. For any random variable  $W = W(t, \mathcal{F}_i)$ , write  $W^{(g)} = W(t, \mathcal{F}_i^{(g)})$  where  $\mathcal{F}_i^{(g)} = (\epsilon_{-\infty}, \dots, \epsilon_{g-1}, \epsilon'_g, \epsilon_{g+1}, \dots, \epsilon_i)$  where  $(\epsilon'_i)_{i \in \mathbb{Z}}$  is an iid copy of  $(\epsilon_i)_{i \in \mathbb{Z}}$ . Let  $\mathcal{P}_j = \mathbb{E}(\cdot | \mathcal{F}_j) - \mathbb{E}(\cdot | \mathcal{F}_{j-1})$  be the projection operator. In the proof, let  $C$  be a generic constant whose value may vary from line to line. Let  $a_{uv}(t) = 0$  if  $v \notin \{l_1, \dots, l_{d(t)}\}$ , where  $l_i, 1 \leq i \leq d(t)$  is the index set of factors defined in Section 1.

**Proof of Theorem ??.**

Notice that for each  $k \in 1, \dots, k_0$ , we have that

$$\sup_{t \in [0,1]} \|\hat{\mathbf{M}}(J_n, t, k) \hat{\mathbf{M}}^\top(J_n, t, k) - \Sigma_X(t, k) \Sigma_X^\top(t, k)\|_F \leq \quad (\text{E.1})$$

$$2\|\Sigma_X^\top(t, k)\|_F \|\hat{\mathbf{M}}(J_n, t, k) - \Sigma_X^\top(t, k)\|_F + \|\hat{\mathbf{M}}(J_n, t, k) - \Sigma_X^\top(t, k)\|_F^2.$$

Notice that by Jansen's inequality, Cauchy-Schwarz inequality and conditions (C1), (M2), (S1)–(S4), it follows that uniformly for  $t \in [0, 1]$ ,

$$\begin{aligned} \|\Sigma_X(t, k)\|_F^2 &\leq 2 \sum_{u=1}^p \sum_{v=1}^p \left( \sum_{u'=1}^d \sum_{v'=1}^d a_{uu'}(t) \mathbb{E}(Q_{u'}(t, \mathcal{F}_{i+k}) Q_{v'}(t, \mathcal{F}_i)) a_{vv'}(t) \right)^2 + 2\|A(t) \Sigma_{z,e}(t, k)\|_F \\ &\leq C \sum_{u=1}^p \sum_{v=1}^p \left[ \sum_{u'=1}^d \sum_{v'=1}^d a_{uu'}(t) a_{vv'}(t) \right]^2 + o(p^{2-2\delta}) \leq C' d^2 p^{2-2\delta}. \end{aligned} \quad (\text{E.2})$$

for some sufficiently large constant  $C$  and  $C'$  which depend on the constant  $M$  in condition (M2). On the other hand, by Lemmas E.4, E.5 and E.6 we have that

$$\left\| \sup_{t \in [0,1]} \|\hat{\mathbf{M}}(J_n, t, k) - \Sigma_X(t, k)\|_F \right\|_{\mathcal{L}^2} = O\left(\frac{J_n p \sup_{t, 1 \leq j \leq J_n} |B_j(t)|^2}{\sqrt{n}} + \beta_n\right). \quad (\text{E.3})$$

Then the theorem follows from equations (E.1), (E.2) and (E.3).  $\square$

### Proof of Theorem ??.

We first prove (i). It suffices to show that the  $d(t)_{th}$  largest eigenvalue of  $\mathbf{\Lambda}(t)$  satisfies

$$\inf_{t \in \mathcal{T}} \lambda_{d(t)}(\mathbf{\Lambda}(t)) \gtrsim \eta_n p^{2-2\delta}. \quad (\text{E.4})$$

Then the theorem follows from Theorem ??, (E.4) and Theorem 1 of Yu et al. (2015). We now show (E.4). Consider the QR decomposition of  $\mathbf{A}(t)$  such that  $\mathbf{A}(t) = \mathbf{V}(t) \mathbf{R}(t)$  where  $\mathbf{V}(t)^\top \mathbf{V}(t) = I_{d(t)}$  and  $I_{d(t)}$  is an  $d(t) \times d(t)$  identity matrix. Here  $\mathbf{V}(t)$  is a  $p \times d(t)$  matrix and  $\mathbf{R}(t)$  is a  $d(t) \times d(t)$  matrix. Then (??) of the main article can be written as

$$\mathbf{\Lambda}(t) = \mathbf{V}(t) \tilde{\mathbf{\Lambda}}(t) \mathbf{V}^\top(t), \quad (\text{E.5})$$

where

$$\tilde{\mathbf{\Lambda}}(t) = \mathbf{R}(t) \left[ \sum_{k=1}^{k_0} (\mathbf{\Sigma}_z(t, k) \mathbf{A}^\top(t) + \mathbf{\Sigma}_{z,e}(t, k)) (\mathbf{A}(t) \mathbf{\Sigma}_z^\top(t, k) + \mathbf{\Sigma}_{z,e}^\top(t, k)) \right] \mathbf{R}^\top(t), \quad (\text{E.6})$$

We now discuss the  $\lambda_{d(t)}(\tilde{\mathbf{\Lambda}}(t))$ . Write

$$\mathbf{\Sigma}_{Rz}(t, k) = \mathbf{R}(t) \mathbf{\Sigma}_z(t, k) \mathbf{R}^\top(t), \mathbf{\Sigma}_{Rz,e}(t, k) = \mathbf{R}(t) \mathbf{\Sigma}_{z,e}(t, k), \quad (\text{E.7})$$

$$\mathbf{\Sigma}_{Rz}^*(t, k_0) = (\mathbf{\Sigma}_{Rz}(t, 1), \dots, \mathbf{\Sigma}_{Rz}(t, k_0)), \mathbf{\Sigma}_{Rz,e}^*(t, k_0) = (\mathbf{\Sigma}_{Rz,e}(t, 1), \dots, \mathbf{\Sigma}_{Rz,e}(t, k_0)). \quad (\text{E.8})$$

Therefore we have

$$\tilde{\mathbf{\Lambda}}(t) = (\mathbf{\Sigma}_{Rz}^*(t, k_0) (I_{k_0} \otimes \mathbf{V}^\top(t)) + \mathbf{\Sigma}_{Rz,e}^*(t, k_0)) (\mathbf{\Sigma}_{Rz}^*(t, k_0) (I_{k_0} \otimes \mathbf{V}^\top(t)) + \mathbf{\Sigma}_{Rz,e}^*(t, k_0))^\top \quad (\text{E.9})$$

where  $\otimes$  denotes the Kronecker product. On the other hand, by (C1) we have

$$\sup_{t \in [0,1]} \|\mathbf{R}(t)\|_2 \asymp p^{\frac{1-\delta}{2}}, \inf_{t \in [0,1]} \|\mathbf{R}(t)\|_2 \asymp p^{\frac{1-\delta}{2}}, \sup_{t \in \mathcal{T}_{\eta_n}} \|\mathbf{R}(t)\|_m \gtrsim \eta_n p^{\frac{1-\delta}{2}}, \inf_{t \in \mathcal{T}_{\eta_n}} \|\mathbf{R}(t)\|_m \gtrsim \eta_n p^{\frac{1-\delta}{2}}.$$

Then by conditions (M1), (M2), (M3), (S2) and (S4) we have

$$\begin{aligned} \sup_{t \in [0,1]} \|\mathbf{\Sigma}_{Rz,e}^*(t, k_0)\|_2 &= o(p^{1-\delta}), \inf_{t \in [0,1]} \|\mathbf{\Sigma}_{Rz,e}^*(t, k_0)\|_2 = o(p^{1-\delta}), \\ \sup_{t \in \mathcal{T}_{\eta_n}} \sigma_{d(t)}(\mathbf{\Sigma}_{Rz}^*(t, k_0)) &\gtrsim \eta_n p^{1-\delta}, \inf_{t \in \mathcal{T}_{\eta_n}} \sigma_{d(t)}(\mathbf{\Sigma}_{Rz}^*(t, k_0)) \gtrsim \eta_n p^{1-\delta}, \end{aligned}$$

where  $\sigma_{d(t)}(\mathbf{\Sigma})$  of a matrix  $\mathbf{\Sigma}$  denotes the  $d(t)_{th}$  singular value of the matrix  $\mathbf{\Sigma}$ . Therefor using the arguments in the proof of Theorem 1 of Lam et al. (2011) we have that

$$\inf_{t \in \mathcal{T}_{\eta_n}} \lambda_{d(t)}(\tilde{\mathbf{\Lambda}}(t)) \gtrsim \eta_n p^{2-2\delta}. \quad (\text{E.10})$$

This shows (E.4). Therefore the (i) of the Theorem follows. The assertion (ii) follows from result (i), condition (C1) and a similar argument of proof of Theorem 3 of Lam et al. (2011). Details are omitted for the sake of brevity.  $\square$

The following lemma from Bhatia (1982) is useful for proving Theorem ??.

**Lemma E.1.** *Let  $M(n)$  be the space of all  $n \times n$  (complex) matrices. A norm  $\|\cdot\|$  on  $M(n)$  is said to be unitary-invariant if  $\|A\| = \|UAV\|$  for any two unitary matrices  $U$  and  $V$ . We denote by  $\text{Eig } A$  the unordered  $n$ -tuple consisting of the eigenvalues of  $A$ , each counted as many times as its multiplicity. Let  $D(A)$  be a diagonal matrix whose diagonal entries are the elements of  $\text{Eig } A$ . For any norm on  $M(n)$  define*

$$\|(\text{Eig } A, \text{Eig } B)\| = \min_W \|D(A) - WD(B)W^{-1}\|$$

where the minimum is taken over all permutation matrices  $W$ . If  $A, B$  are Hermitian matrices, we have for all unitary-invariant norms (including the Frobenius norm) the inequality

$$\|(\text{Eig } A, \text{Eig } B)\| \leq \|A - B\|.$$

**Proof of Theorem ??.** (i) follows immediately from Lemma E.1 and Theorem ??. For (ii), notice that by Theorem ?? we have that

$$\left\| \sup_{t \in \mathcal{T}_{\eta_n}} \|\hat{\mathbf{B}}(t) - \mathbf{B}(t)\hat{\mathbf{O}}_2^\top(t)\|_F \right\|_{\mathcal{L}^1} = O \left( \eta_n^{-1} p^{\delta-1} \left( \frac{J_n p \sup_{j,t} |B_j(t)|^2}{\sqrt{n}} + \beta_n \right) \right), \quad (\text{E.11})$$

where  $\mathbf{B}(t)$ ,  $\hat{\mathbf{B}}(t)$  and  $\hat{\mathbf{O}}_2(t)$  are defined in Theorem ??. Since  $\hat{\mathbf{O}}_2(t)$  is an  $(p - d(t)) \times (p - d(t))$  orthonormal matrix, it is easy to check that  $\mathbf{B}(t)\hat{\mathbf{O}}_2^\top(t)$  is an orthonormal basis of the null space of  $\mathbf{\Lambda}(t)$ . Using this fact, we then follow the decomposition (A.5) of Lam and Yao (2012) to obtain that uniformly for  $j = d(t) + 1, \dots, p$

$$\lambda_j(\hat{\mathbf{\Lambda}})(t) = K_{1,j}(t) + K_{2,j}(t) + K_{3,j}(t), \quad (\text{E.12})$$

with

$$\sup_{t \in \mathcal{T}_{\eta_n}} |K_{1,j}(t)| \leq \sum_{k=1}^{k_0} \sup_{t \in \mathcal{T}_{\eta_n}} \|\hat{\mathbf{M}}(J_n, t, k) - \mathbf{\Sigma}_X(t, k)\|_F^2, \quad (\text{E.13})$$

$$\sup_{t \in \mathcal{T}_{\eta_n}} |K_{2,j}(t)| \leq M_1 \sup_{t \in \mathcal{T}_{\eta_n}} \|\hat{\mathbf{\Lambda}}(t) - \mathbf{\Lambda}(t)\|_F \|\hat{\mathbf{B}}(t) - \mathbf{B}(t)\hat{\mathbf{O}}_2^\top(t)\|_F, \quad (\text{E.14})$$

$$\sup_{t \in \mathcal{T}_{\eta_n}} |K_{3,j}(t)| \leq M_2 \|\hat{\mathbf{B}}(t) - \mathbf{B}(t)\hat{\mathbf{O}}_2^\top(t)\|_F^2 \|\mathbf{\Lambda}(t)\|_F \quad (\text{E.15})$$

for some sufficiently large constants  $M_1$  and  $M_2$ . Notice that the RHS of the above inequalities are independent of  $j$ . By (E.3), for  $K_{1,j}(t)$  we have that

$$\left\| \sup_{t \in \mathcal{T}_{\eta_n}} \max_{d(t)+1 \leq j \leq p} |K_{1,j}(t)| \right\|_{\mathcal{L}^1} = O \left( \left( \frac{J_n p \sup_{j,t} |B_j(t)|^2}{\sqrt{n}} + \beta_n \right)^2 \right). \quad (\text{E.16})$$

Notice that for any two random variables  $X, Y$  with finite first moments, for any  $c > 0$ , the following inequality holds by Markov inequality

$$\mathbb{P}(|XY| \geq c^2 \mathbb{E}|X| \mathbb{E}|Y|) \leq \mathbb{P}(|X| \geq c \mathbb{E}|X|) + \mathbb{P}(|Y| \geq c \mathbb{E}|Y|) \leq 2/c. \quad (\text{E.17})$$

Notice that  $\eta_n^{-1} \left( \frac{J_n p \sup_{j,t} |B_j(t)|^2}{\sqrt{n}} + \beta_n \right)^2 = \eta_n^{-1} p^{1-\delta} \left( \frac{J_n p \sup_{j,t} |B_j(t)|^2}{\sqrt{n}} + \beta_n \right) p^{\delta-1} \left( \frac{J_n p \sup_{j,t} |B_j(t)|^2}{\sqrt{n}} + \beta_n \right)$ . Therefor by (E.17) and the results of Theorem ??, Theorem ?? and the upperbound of  $K_{2,j}(t)$ , we have that

$$\mathbb{P} \left( \sup_{t \in \mathcal{T}_{\eta_n}} \max_{d(t)+1 \leq j \leq p} |K_{2,j}(t)| \geq \eta_n^{-1} \left( \frac{J_n p \sup_{j,t} |B_j(t)|^2}{\sqrt{n}} + \beta_n \right)^2 g_n^2 \right) = O(1/g_n). \quad (\text{E.18})$$

By (E.2) we shall see that

$$\sup_{t \in \mathcal{T}_{\eta_n}} \|\mathbf{\Lambda}(t)\|_F \asymp p^{2-2\delta}, \quad (\text{E.19})$$

which together with Theorem ?? and (E.17) provides the probabilistic bound for  $K_{3,j}(t)$

$$\mathbb{P} \left( \sup_{t \in \mathcal{T}_{\eta_n}} \max_{d(t)+1 \leq j \leq p} |K_{3,j}(t)| \geq g_n^2 \eta_n^{-2} \left( \frac{J_n p \sup_{j,t} |B_j(t)|^2}{\sqrt{n}} + \beta_n \right)^2 \right) = O(1/g_n). \quad (\text{E.20})$$

As a result, (ii) follows from (E.16), (E.18) and (E.20).

For (iii), notice that by (E.10) and (E.19) it follows that

$$\inf_{t \in \mathcal{T}_{\eta_n}} \|\mathbf{\Lambda}(t)\|_m \gtrsim \eta_n p^{2-2\delta}, \sup_{t \in \mathcal{T}_{\eta_n}} \|\mathbf{\Lambda}(t)\|_m \lesssim \eta_n p^{2-2\delta}, \inf_{t \in \mathcal{T}_{\eta_n}} \|\mathbf{\Lambda}(t)\|_2 \asymp p^{2-2\delta}, \sup_{t \in \mathcal{T}_{\eta_n}} \|\mathbf{\Lambda}(t)\|_2 \asymp p^{2-2\delta}. \quad (\text{E.21})$$

Then by (i)

$$\mathbb{P}\left(\frac{\lambda_{j+1}(\hat{\mathbf{\Lambda}}(t))}{\lambda_j(\hat{\mathbf{\Lambda}}(t))} \geq \eta_n, j = 1, \dots, d(t) - 1, \forall t \in \mathcal{T}_{\eta_n}\right) \geq \mathbb{P}\left(\sup_{t \in \mathcal{T}_{\eta_n}} \max_{1 \leq j \leq d(t)} |\lambda_j(\hat{\mathbf{\Lambda}}(t)) - \lambda_j(\mathbf{\Lambda}(t))| \leq \frac{\eta_n p^{2-2\delta}}{\tilde{M}_0}\right), \quad (\text{E.22})$$

where  $\tilde{M}_0$  is a sufficiently large constant such that  $\eta_n p^{2-2\delta} / \tilde{M}_0 < 1/2 \inf_{t \in \mathcal{T}_{\eta_n}} \lambda_{d(t)}(\mathbf{\Lambda}(t))$ . Therefore by (i) and Markov inequality (iii) holds. Finally, (iv) follows from (i), (ii), (E.21) and (E.17).  $\square$

**Proof of Proposition ??.** Consider  $g_n = \frac{\eta_n^2}{\nu_n p^{\delta-1} \log n}$ . Then the conditions of Theorem ?? hold. Since  $\sum_{j=1}^p \lambda_j^2(\hat{\mathbf{\Lambda}}(t)) = \|\hat{\mathbf{\Lambda}}(t)\|_F^2$ , we shall discuss the magnitude of  $\|\hat{\mathbf{\Lambda}}(t)\|_F$ . First, notice that by using similar and simpler argument of proofs of Theorem ?? it follows that  $\inf_{t \in \mathcal{T}_{\eta_n}} \|\mathbf{\Lambda}(t)\|_F \asymp p^{2-2\delta}$ . By Theorem ?? and (E.19) we shall see that

$$\sup_{t \in \mathcal{T}_{\eta_n}} \|\hat{\mathbf{\Lambda}}(t)\|_F \asymp p^{2-2\delta}, \quad \inf_{t \in \mathcal{T}_{\eta_n}} \|\hat{\mathbf{\Lambda}}(t)\|_F \asymp p^{2-2\delta}. \quad (\text{E.23})$$

Define the events

$$A_n = \left\{ \sup_{t \in \mathcal{T}_{\eta_n}} \max_{1 \leq j \leq d(t)} |\lambda_j(\hat{\mathbf{\Lambda}}(t)) - \lambda_j(\mathbf{\Lambda}(t))| \leq \frac{\eta_n p^{2-2\delta}}{\tilde{M}_0} \right\}, \quad B_n = \left\{ \sup_{t \in \mathcal{T}_{\eta_n}} \frac{\lambda_{d(t)+1}(\hat{\mathbf{\Lambda}}(t))}{\lambda_{d(t)}(\hat{\mathbf{\Lambda}}(t))} \geq p^{2\delta-2} g_n^2 \nu_n^2 / \eta_n^3 \right\}. \quad (\text{E.24})$$

By the proof of Theorem ??, we shall see that

$$\mathbb{P}(A_n) = 1 - O\left(\frac{\nu_n}{\eta_n p^{1-\delta}}\right), \quad \mathbb{P}(B_n) = 1 - O(1/g_n) - O\left(\frac{\nu_n}{\eta_n p^{1-\delta}}\right). \quad (\text{E.25})$$

Notice that on  $A_n$ , by the choice of  $R(t)$ ,

$$\begin{aligned} \inf_{t \in \mathcal{T}_{\eta_n}} \min_{d(t)+1 \leq j \leq R(t)} \frac{\lambda_{j+1}(\hat{\mathbf{\Lambda}}(t))}{\lambda_j(\hat{\mathbf{\Lambda}}(t))} &\geq \inf_{t \in \mathcal{T}_{\eta_n}} \min_{d(t)+1 \leq j \leq R(t)} \frac{\lambda_{j+1}(\hat{\mathbf{\Lambda}}(t))}{\lambda_{d(t)}(\hat{\mathbf{\Lambda}}(t))} \geq C_0 \frac{\eta_n p^{2-2\delta}}{\eta_n p^{2-2\delta} \log n} \\ &= C_0 / \log n \end{aligned} \quad (\text{E.26})$$

for some sufficiently small positive constant  $C_0$ , where the last  $\geq$  is due to (E.23). Because on  $A_n$ ,  $\inf_{t \in \mathcal{T}_{\eta_n}} \min_{1 \leq j \leq d(t)} \frac{\lambda_{j+1}(\hat{\mathbf{\Lambda}}(t))}{\lambda_j(\hat{\mathbf{\Lambda}}(t))} \geq \eta_n$  (c.f.(E.22)), and the fact that  $p^{2\delta-2} g_n^2 \nu_n^2 / \eta_n^3 = o(\min(\eta_n, (\log n)^{-1}))$ ,

we have that

$$\mathbb{P}(\hat{d}_n(t) = d(t), \forall t \in \mathcal{T}_{\eta_n}) \geq \mathbb{P}(A_n \cap B_n) = 1 - O\left(\frac{1}{g_n}\right) - O\left(\frac{\nu_n}{\eta_n p^{1-\delta}}\right). \quad (\text{E.27})$$

Therefore the Proposition holds by considering  $g_n = \frac{\eta_n^2}{\nu_n p^{\delta-1} \log n}$ .  $\square$

## 5.1 Auxiliary Lemmas

**Lemma E.2.** *Recall in the main article that*

$$\delta_{G,l}(k) = \sup_{t \in [0,1], i \in \mathbb{Z}, 1 \leq j \leq p} \|G_j(t, \mathcal{F}_i) - G_j(t, \mathcal{F}_i^{(i-k)})\|_{\mathcal{L}^1}. \quad (\text{E.28})$$

*Under conditions (A1), and (M1)–(M3), there exists a sufficiently large constant  $M_0$ , such that uniformly for  $1 \leq u \leq p$  and  $t \in [0, 1]$ ,*

$$\mathbb{E}|G_u(t, \mathcal{F}_0)|^4 \leq M_0, \quad (\text{E.29})$$

$$\delta_{G,l}(k) = O(d\delta_{Q,l}(k) + \delta_{H,l}(k)). \quad (\text{E.30})$$

*Proof.* By definition we have that for  $1 \leq u \leq p$ ,

$$G_u(t, \mathcal{F}_i) = \sum_{v=1}^d a_{uv}(t) Q_v(t, \mathcal{F}_i) + H_u(t, \mathcal{F}_i).$$

Notice that  $d = \sup_{0 \leq t \leq 1} d(t)$  is fixed. Therefore, assumptions (A1), (M2) and triangle inequality lead to the first statement of boundedness of fourth moment of (E.29). Finally (A1) and (M3) lead to the assertion (E.30).  $\square$

**Lemma E.3.** *Consider the process  $z_{i,u,n} z_{i+k,v,n}$  for some  $k > 0$ , and  $1 \leq u, v \leq d$ . Then under conditions (C1), (M1)–(M3) we have i)  $\zeta_{i,u,v} =: \zeta_{u,v}(\frac{i}{n}, \mathcal{F}_i) = z_{i,u,n} z_{i+k,v,n}$  is a locally stationary process with associated dependence measures*

$$\delta_{\zeta_{u,v},2}(h) \leq C(\delta_{Q,4}(h) + \delta_{Q,4}(h+k)) \quad (\text{E.31})$$

*for some universal constant  $C > 0$  independent of  $u, v$  and any integer  $h$ ; (ii) For any series of*

numbers  $a_i, 1 \leq i \leq n$ , we have

$$\left( \mathbb{E} \left| \frac{1}{n} \sum_{i=1}^n a_i (\zeta_{i,u,v} - \mathbb{E} \zeta_{i,u,v}) \right|^2 \right)^{1/2} \leq \frac{2C}{n} \left( \sum_{i=1}^n a_i^2 \right)^{\frac{1}{2}} \Delta_{Q,4,0}. \quad (\text{E.32})$$

*Proof.* i) is a consequence of the Cauchy-Schwarz inequality, triangle inequality and conditions (M1), (M2). For ii), notice that

$$\sum_{i=1}^n a_i (\zeta_{i,u,v} - \mathbb{E} \zeta_{i,u,v}) = \sum_{i=1}^n a_i \left( \sum_{u=0}^{\infty} \mathcal{P}_{i+k-u} \zeta_{i,u,v} \right) = \sum_{u=0}^{\infty} \sum_{i=1}^n a_i \mathcal{P}_{i+k-u} \zeta_{i,u,v}. \quad (\text{E.33})$$

By the property of martingale difference and i) of this lemma we have

$$\left\| \sum_{i=1}^n a_i \mathcal{P}_{i+k-u} \zeta_{i,u,v} \right\|_{\mathcal{L}^2} = \sum_{i=1}^n a_i^2 \left\| \mathcal{P}_{i+k-u} \zeta_{i,u,v} \right\|_{\mathcal{L}^2}^2 \leq C^2 \sum_{i=1}^n a_i^2 (\delta_{Q,4}(u) + \delta_{Q,4}(u-k))^2. \quad (\text{E.34})$$

By triangle inequality, inequalities (E.33) and (E.34), the lemma follows.  $\square$

**Corollary 5.1.** *Under conditions (C1), (M1) and (M2) we have for each fixed  $k > 0$ ,  $1 \leq u, v \leq p$  and  $1 \leq w \leq d$ , i)  $\psi_i =: \psi(\frac{i}{n}, \mathcal{F}_i) = e_{i+k,u,n} e_{i,v,n}$ ,  $\phi_i =: \phi(\frac{i}{n}, \mathcal{F}_i) = z_{i+k,w,n} e_{i,v,n}$  and  $\iota_i =: \iota(\frac{i}{n}, \mathcal{F}_i) = e_{i+k,u,n} z_{i,w,n}$  are locally stationary processes with associated dependence measures*

$$\max(\delta_{\psi,2}(h), \delta_{\phi,2}(h), \delta_{\iota,2}(h)) \leq C(\delta_{Q,4}(h) + \delta_{H,4}(h) + \delta_{Q,4}(h+k) + \delta_{H,4}(h+k)). \quad (\text{E.35})$$

for some universal constant  $C > 0$  independent of  $u, v$  and  $w$ .

*Proof.* The corollary follows from the same proof of Lemma E.3.  $\square$

To save notation in the following proofs, for given  $J_n, k$  write  $\hat{\mathbf{M}}(J_n, t, k)$  as  $\hat{\mathbf{M}}$  if no confusion arises. Recall the definition of  $\tilde{\Sigma}_{X,j,k}$  and  $\hat{\mathbf{M}}(J_n, t, k)$  in (??) and (??) in the main article. Observe the following decompositions

$$\tilde{\Sigma}_{X,j,k} = \mathbf{V}_{1,j,k} + \mathbf{V}_{2,j,k} + \mathbf{V}_{3,j,k} + \mathbf{V}_{4,j,k}, \quad (\text{E.36})$$

$$\mathbf{V}_{1,j,k} = \frac{1}{n} \sum_{i=1}^{n-k} \mathbf{A} \left( \frac{i+k}{n} \right) \mathbf{z}_{i+k,n} \mathbf{z}_{i,n}^{\top} \mathbf{A}^{\top} \left( \frac{i}{n} \right) B_j \left( \frac{i}{n} \right), \quad (\text{E.37})$$

$$\mathbf{V}_{2,j,k} = \frac{1}{n} \sum_{i=1}^{n-k} \mathbf{A} \left( \frac{i+k}{n} \right) \mathbf{z}_{i+k,n} \mathbf{e}_{i,n}^{\top} B_j \left( \frac{i}{n} \right), \quad (\text{E.38})$$

$$\mathbf{V}_{3,j,k} = \frac{1}{n} \sum_{i=1}^{n-k} \mathbf{e}_{i+k} \mathbf{z}_{i,n}^\top \mathbf{A}(\frac{i}{n}) B_j(\frac{i}{n}), \mathbf{V}_{4,j,k} = \frac{1}{n} \sum_{i=1}^{n-k} \mathbf{e}_{i+k,n} \mathbf{e}_{i,n}^\top B_j(\frac{i}{n}). \quad (\text{E.39})$$

**Lemma E.4.** *Under conditions (C1) and (M1), (M2) and (M3) we have that*

$$\| \sup_{t \in [0,1]} \|\hat{\mathbf{M}}(J_n, t, k) - \mathbb{E}\hat{\mathbf{M}}(J_n, t, k)\|_F \|_{\mathcal{L}^2} = O\left(\frac{J_n p \sup_{t, 1 \leq j \leq J_n} |B_j(t)|^2}{\sqrt{n}}\right).$$

*Proof.* Using equations (E.36)-(E.39) we have that

$$\hat{\mathbf{M}}(J_n, t, k) - \mathbb{E}\hat{\mathbf{M}}(J_n, t, k) = \sum_{j=1}^{J_n} \sum_{s=1}^4 (\mathbf{V}_{s,j,k} - \mathbb{E}(\mathbf{V}_{s,j,k})) B_j(t) := \sum_{s=1}^4 \tilde{\mathbf{V}}_s(t), \quad (\text{E.40})$$

where  $\tilde{\mathbf{V}}_s(t) = \sum_{j=1}^{J_n} (\mathbf{V}_{s,j,k} - \mathbb{E}(\mathbf{V}_{s,j,k})) B_j(t)$ , for  $s = 1, 2, 3, 4$ . Consider the  $s = 1$  case and then

$$\begin{aligned} \tilde{\mathbf{V}}_1(t) &:= \sum_{j=1}^{J_n} (\mathbf{V}_{1,j,k} - \mathbb{E}(\mathbf{V}_{1,j,k})) B_j(t) \\ &= \frac{1}{n} \sum_{j=1}^{J_n} B_j(t) \sum_{i=1}^{n-k} \mathbf{A}(\frac{i+k}{n}) (\mathbf{z}_{i+k,n} \mathbf{z}_{i,n}^\top - \mathbb{E}(\mathbf{z}_{i+k,n} \mathbf{z}_{i,n}^\top)) \mathbf{A}^\top(\frac{i}{n}) B_j(\frac{i}{n}). \end{aligned} \quad (\text{E.41})$$

Consider  $\tilde{\mathbf{M}}_j = \frac{1}{n} \sum_{i=1}^{n-k} \mathbf{A}(\frac{i+k}{n}) (\mathbf{z}_{i+k,n} \mathbf{z}_{i,n}^\top - \mathbb{E}(\mathbf{z}_{i+k,n} \mathbf{z}_{i,n}^\top)) \mathbf{A}^\top(\frac{i}{n}) B_j(\frac{i}{n})$ . Its  $(u, v)_{th}$ ,  $1 \leq u \leq p$ ,  $1 \leq v \leq p$  element is

$$\tilde{M}_{j,u,v} = \frac{1}{n} \sum_{i=1}^{n-k} \sum_{u'=1}^d \sum_{v'=1}^d a_{uu'}(\frac{i+k}{n}) (z_{i+k,u',n} z_{i,v',n} - \mathbb{E}(z_{i+k,u',n} z_{i,v',n})) a_{vv'}(\frac{i}{n}) B_j(\frac{i}{n}). \quad (\text{E.42})$$

Therefore it follows from the triangle inequality and Lemma E.3 that,

$$\|\tilde{M}_{j,u,v}\|_{\mathcal{L}^2} \leq \frac{C \Delta_{Q,4,0} \sup_{j,t} |B_j(t)|}{n} \sum_{v'=1}^d \sum_{u'=1}^d \sqrt{\sum_{i=1}^{n-k} a_{uu'}^2(\frac{i+k}{n}) a_{vv'}^2(\frac{i}{n})} \quad (\text{E.43})$$

for some sufficiently large constant  $C$ . Consequently by (C1) and Jansen's inequality, we get

$$\mathbb{E} \left( \|\tilde{\mathbf{M}}_j\|_F^2 \right) \leq \frac{C^2 \Delta_{Q,4,0}^2 \sup_{j,t} |B_j(t)|^2}{n^2} \sum_{u=1}^p \sum_{v=1}^p \left( \sum_{v'=1}^d \sum_{u'=1}^d \sqrt{\sum_{i=1}^{n-k} a_{uu'}^2(\frac{i+k}{n}) a_{vv'}^2(\frac{i}{n})} \right)^2$$

$$\begin{aligned}
&\leq \frac{C^2 \Delta_{Q,4,0}^2 d^2 \sup_{j,t} |B_j(t)|^2}{n^2} \sum_{i=1}^{n-k} \sum_{u=1}^p \sum_{v=1}^p \sum_{v'=1}^d \sum_{u'=1}^d a_{uu'}^2 \left(\frac{i+k}{n}\right) a_{vv'}^2 \left(\frac{i}{n}\right) \\
&\asymp \frac{\Delta_{Q,4,0}^2 d^4 \sup_{j,t} |B_j(t)|^2 p^{2-2\delta}}{n}
\end{aligned} \tag{E.44}$$

for  $1 \leq j \leq J_n$ . On the other hand, since  $(u, v)_{th}$  element of  $\tilde{\mathbf{V}}_1(t)$ , which is denoted by  $\tilde{V}_{1,u,v}(t)$ , satisfies

$$\tilde{V}_{1,u,v}(t) = \frac{1}{n} \sum_{j=1}^{J_n} B_j(t) \tilde{M}_{j,u,v}. \tag{E.45}$$

Therefore by Jansen's inequality it follows that

$$\begin{aligned}
\sup_{t \in [0,1]} \|\tilde{\mathbf{V}}_1(t)\|_F^2 &= \sup_{t, 1 \leq j \leq J_n} \sum_{u=1}^p \sum_{v=1}^p \left( \sum_{j=1}^{J_n} B_j(t) \tilde{M}_{j,u,v} \right)^2 \\
&\leq \sup_{t, 1 \leq j \leq J_n} |B_j(t)|^2 \sum_{u=1}^p \sum_{v=1}^p \left( \sum_{j=1}^{J_n} |\tilde{M}_{j,u,v}| \right)^2 \\
&\leq \sup_{t, 1 \leq j \leq J_n} |B_j(t)|^2 \sum_{u=1}^p \sum_{v=1}^p J_n \sum_{j=1}^{J_n} |\tilde{M}_{j,u,v}|^2 \\
&\leq \sup_{t, 1 \leq j \leq J_n} |B_j(t)|^2 J_n \sum_{j=1}^{J_n} \|\tilde{\mathbf{M}}_j\|_F^2.
\end{aligned} \tag{E.46}$$

Therefore we have

$$\mathbb{E} \left( \sup_{t \in [0,1]} \|\tilde{\mathbf{V}}_1(t)\|_F^2 \right) \leq \sup_{t, 1 \leq j \leq J_n} |B_j(t)|^2 J_n \sum_{j=1}^{J_n} \mathbb{E}(\|\tilde{\mathbf{M}}_j\|_F^2) \tag{E.47}$$

Combining (E.44) we have that

$$\mathbb{E} \left( \sup_{t \in [0,1]} \|\tilde{\mathbf{V}}_1(t)\|_F^2 \right)^{1/2} = O \left( \frac{J_n \sup_{t, 1 \leq j \leq J_n} |B_j(t)|^2 p^{1-\delta}}{\sqrt{n}} \right). \tag{E.48}$$

Similarly using Corollary 5.1 we have that

$$\mathbb{E} \left( \sup_{t \in [0,1]} \|\tilde{\mathbf{V}}_s(t)\|_F^2 \right)^{\frac{1}{2}} = O \left( \frac{J_n \sup_{t, 1 \leq j \leq J_n} |B_j(t)|^2 p^{1-\delta/2}}{\sqrt{n}} \right), s = 2, 3, \tag{E.49}$$

and

$$\mathbb{E} \left( \sup_{t \in [0,1]} \|\tilde{\mathbf{V}}_4(t)\|_F^2 \right)^{\frac{1}{2}} = O \left( \frac{J_n p \sup_{t, 1 \leq j \leq J_n} |B_j(t)|^2}{\sqrt{n}} \right). \quad (\text{E.50})$$

Then the lemma follows from (E.48), (E.49), (E.50) and triangle inequality.  $\square$

**Lemma E.5.** *Under conditions (A1) (A2), (C1), (M1), (M2) and (M3) we have that*

$$\| \sup_{t \in [0,1]} (\hat{\mathbb{E}}\mathbf{M}(J_n, t, k) - \Sigma_k^*(t)) \|_F = O(J_n \sup_{t, 1 \leq j \leq J_n} |B_j(t)|^2 k p / n)$$

where  $\Sigma_k^*(t) = \frac{1}{n} \sum_{j=1}^{J_n} \sum_{i=1}^n \mathbb{E}(\mathbf{G}(\frac{i}{n}, \mathcal{F}_{i+k}) \mathbf{G}(\frac{i}{n}, \mathcal{F}_i)^\top) B_j(\frac{i}{n}) B_j(t)$ .

*Proof.* Consider the  $(u, v)_{th}$  element of  $(\hat{\mathbb{E}}\mathbf{M}(J_n, t, k) - \Sigma_k^*(t))_{u,v}$ . By definition, we have for  $1 \leq u, v \leq p$ ,

$$\begin{aligned} (\hat{\mathbb{E}}\mathbf{M}(J_n, t, k) - \Sigma_k^*(t))_{uv} &= \frac{1}{n} \sum_{j=1}^{J_n} \sum_{i=1}^{n-k} \mathbb{E} \left( \left( G_u\left(\frac{i+k}{n}, \mathcal{F}_{i+k}\right) - G_u\left(\frac{i}{n}, \mathcal{F}_{i+k}\right) \right) G_v\left(\frac{i}{n}, \mathcal{F}_i\right) \right) B_j\left(\frac{i}{n}\right) B_j(t) \\ &\quad + \frac{1}{n} \sum_{j=1}^{J_n} \sum_{i=n-k+1}^n \mathbb{E} \left( G_u\left(\frac{i}{n}, \mathcal{F}_{i+k}\right) G_v\left(\frac{i}{n}, \mathcal{F}_i\right) \right) B_j\left(\frac{i}{n}\right) B_j(t). \end{aligned} \quad (\text{E.51})$$

By condition (M3) we have that uniformly for  $1 \leq u, v \leq p$ ,

$$\sup_{t \in [0,1]} |(\hat{\mathbb{E}}\mathbf{M}(J_n, t, k) - \Sigma_k^*(t))_{uv}| \leq M' J_n \sup_{t, 1 \leq j \leq J_n} |B_j(t)|^2 k / n \quad (\text{E.52})$$

for some sufficiently large constant  $M'$  independent of  $u$  and  $v$ . Therefore by the definition of Frobenius norm, the lemma follows.  $\square$

**Lemma E.6.** *Let  $\iota_n = \sup_{1 \leq j \leq J_n} \text{Lip}_j + \sup_{t, 1 \leq j \leq J_n} |B_j(t)|$  where  $\text{Lip}_j$  is the Lipschitz constant of the basis function  $B_j(t)$ . Then under conditions (A1), (A2), (C1), (M1)–(M3) we have that*

$$\sup_{t \in [0,1]} \|\Sigma_k^*(t) - \Sigma_X(t, k)\|_F = O \left( \frac{J_n \sup_{t, 1 \leq j \leq J_n} |B_j(t)| p \iota_n}{n} + p g_{J_n, K, \tilde{M}} \right),$$

where  $\Sigma_k^*$  is defined in Lemma E.5.

*Proof.* Notice that by definition we have that

$$\Sigma_k^*(t) = \frac{1}{n} \sum_{j=1}^{J_n} \sum_{i=1}^n \Sigma_X\left(\frac{i}{n}, k\right) B_j\left(\frac{i}{n}\right) B_j(t). \quad (\text{E.53})$$

Define that  $\tilde{\Sigma}_k^*(t) = \sum_{j=1}^{J_n} \int_0^1 \Sigma_X(s, k) B_j(s) ds B_j(t)$ . Notice that the  $(u, v)_{th}$  element of  $\Sigma_k^*(t) - \tilde{\Sigma}_k^*(t)$  is

$$\begin{aligned} (\Sigma_k^*(t) - \tilde{\Sigma}_k^*(t))_{u,v} &= \sum_{j=1}^{J_n} \left( \frac{1}{n} \sum_{i=1}^n \mathbb{E}(G_u\left(\frac{i}{n}, \mathcal{F}_{i+k}\right) G_v\left(\frac{i}{n}, \mathcal{F}_i\right)) B_j\left(\frac{i}{n}\right) \right. \\ &\quad \left. - \int_0^1 \mathbb{E}(G_u(s, \mathcal{F}_{i+k}) G_v(s, \mathcal{F}_i)) B_j(s) ds \right) B_j(t). \end{aligned} \quad (\text{E.54})$$

Notice that Lemma E.2 and Condition (A2) imply that there exists a sufficiently large constant  $M'$  depending on  $M_0$  of Lemma E.2, such that those Lipschitz constants of the functions

$$\mathbb{E}(G_u(s, \mathcal{F}_{i+k}) G_v(s, \mathcal{F}_i)) B_j(s)$$

are bounded by  $M' \iota_n$  for all  $1 \leq k \leq k_0$ ,  $1 \leq u, v \leq p$ . Then using similar argument to the proof of Lemma E.5, we obtain that

$$\sup_{t \in [0,1]} \|\Sigma_k^*(t) - \tilde{\Sigma}_k^*(t)\|_F = O\left(\frac{J_n \sup_{t, 1 \leq j \leq J_n} |B_j(t)| p \iota_n}{n}\right). \quad (\text{E.55})$$

Similarly by using basis expansion (A.2) in condition (A2) have we have that

$$\sup_{t \in [0,1]} \|\tilde{\Sigma}_k^*(t) - \Sigma_X(t, k)\|_F = O(p g_{J_n, K, \tilde{M}}) \quad (\text{E.56})$$

which completes the proof.  $\square$

## 6 Proof of Propositions ?? , ?? and Theorems ??, ??

In this section we define  $\hat{\mathbf{W}}_i$ ,  $i = 1, \dots, d$  as the orthonormal eigenvectors of  $(\lambda_1(\sum_{k=1}^{k_0} \hat{\Gamma}_k), \dots, \lambda_d(\sum_{k=1}^{k_0} \hat{\Gamma}_k))$ . Denote by  $\mathbf{W}_i$ ,  $i = 1, \dots, d$  the orthonormal eigenvectors with respect to the  $d$  positive eigenvalues of  $\sum_{k=1}^{k_0} \Gamma_k$ :  $(\lambda_1(\sum_{k=1}^{k_0} \Gamma_k), \dots, \lambda_d(\sum_{k=1}^{k_0} \Gamma_k))$ . Let  $\mathbf{W} = (\mathbf{W}_1, \dots, \mathbf{W}_d)$ ,  $\mathbf{F} = (\mathbf{F}_1, \dots, \mathbf{F}_{p-d})$ , and sim-

ilarly  $\hat{\mathbf{W}} = (\hat{\mathbf{W}}_1, \dots, \hat{\mathbf{W}}_d)$ ,  $\hat{\mathbf{F}} = (\hat{\mathbf{F}}_1, \dots, \hat{\mathbf{F}}_{p-d})$ . We also require that  $\hat{\mathbf{W}}^\top \hat{\mathbf{F}} = \mathbf{0}$ ,  $\mathbf{W}^\top \mathbf{F} = \mathbf{0}$ , i.e.,  $((\mathbf{W}_i, 1 \leq i \leq d), (\mathbf{F}_i, 1 \leq i \leq p-d))$  and  $((\hat{\mathbf{W}}_i, 1 \leq i \leq d), (\hat{\mathbf{F}}_i, 1 \leq i \leq p-d))$  are both orthonormal basis for  $\mathbb{R}^p$ . Notice that  $\hat{\mathbf{\Gamma}}(t) = \sum_{k=1}^{k_0} \hat{\mathbf{\Gamma}}_k$  and  $\mathbf{\Gamma} = \sum_{k=1}^{k_0} \mathbf{\Gamma}_k$ .

Since we are testing the null hypothesis of static factor loadings and are considering local alternatives where  $\mathbf{A}(\cdot)$  deviates slightly from the null in this section, we assume throughout this section that  $d(t) \equiv d$ , i.e., the number of factors is fixed. Because in this section it is assumed that there are no change points in the number of factors, we can assume that  $\eta_n$  in conditions (C1), (S) satisfies  $\eta_n \geq \eta_0 > 0$  for some positive constant  $\eta_0$ , and  $\mathcal{T}_{\eta_n} = (0, 1)$  which coincides with discussions in Remark ?? of the main article.

**Corollary F.1.** *Assume (A1), (A2), (C1), (M1)–(M3).*

$$\|\|\mathbf{\Gamma} - \hat{\mathbf{\Gamma}}\|_F\|_{\mathcal{L}^1} = O\left(\frac{p^{2-\delta}}{\sqrt{n}}\right) \quad (\text{F.1})$$

*Proof.* It suffices to show uniformly for  $1 \leq k \leq k_0$ ,

$$\|\|\mathbf{\Gamma}_k - \hat{\mathbf{\Gamma}}_k\|_F\|_{\mathcal{L}^1} = O_p\left(\frac{p^{2-\delta}}{\sqrt{n}}\right) \quad (\text{F.2})$$

By the proof of Lemma E.4, it follows that for  $1 \leq k \leq k_0$ ,

$$\left\|\left\|\frac{1}{n} \sum_{i=1}^{n-k} \mathbf{X}_{i+k,n} \mathbf{X}_{i,n}^\top - \frac{1}{n} \mathbb{E}\left(\sum_{i=1}^{n-k} \mathbf{X}_{i+k,n} \mathbf{X}_{i,n}^\top\right)\right\|_F\right\|_{\mathcal{L}^2} = O\left(\frac{p}{\sqrt{n}}\right). \quad (\text{F.3})$$

By the proof of Lemma E.5, it follows that

$$\left\|\frac{1}{n} \sum_{i=1}^{n-k} \left(\mathbb{E}(\mathbf{X}_{i+k,n} \mathbf{X}_{i,n}^\top) - \Sigma_X\left(\frac{i}{n}, k\right)\right)\right\|_F = O\left(\frac{p}{n}\right), \quad (\text{F.4})$$

$$\left\|\frac{1}{n} \sum_{i=1}^{n-k} \Sigma_X\left(\frac{i}{n}, k\right) - \int_0^1 \Sigma_X(t, k) dt\right\|_F = O\left(\frac{p}{n}\right), \quad (\text{F.5})$$

where to prove (F.5) we have used Lemma E.2. Then by (F.3) to (F.5) we have that

$$\left\|\frac{1}{n} \sum_{i=1}^{n-k} \mathbf{X}_{i+k,n} \mathbf{X}_{i,n}^\top - \int_0^1 \Sigma_X(t, k) dt\right\|_F = O\left(\frac{p}{\sqrt{n}}\right), \quad (\text{F.6})$$

which together with (E.2) and the definition of  $\mathbf{\Gamma}_k$  proves (F.2). Therefore the corollary holds.  $\square$

**Corollary F.2.** *Assume conditions (A1), (A2), (C1), (M1), (M2), (M3) and condition (S1)-(S4), then there exists orthogonal matrices  $\hat{\mathbf{O}}_3 \in \mathbb{R}^{d \times d}$ ,  $\hat{\mathbf{O}}_4 \in \mathbb{R}^{(p-d) \times (p-d)}$  such that*

$$\begin{aligned} \|\|\hat{\mathbf{W}}\hat{\mathbf{O}}_3 - \mathbf{W}\|_F\|_{\mathcal{L}^1} &= O\left(\frac{p^\delta}{\sqrt{n}}\right), \\ \|\|\hat{\mathbf{F}}\hat{\mathbf{O}}_4 - \mathbf{F}\|_F\|_{\mathcal{L}^1} &= O\left(\frac{p^\delta}{\sqrt{n}}\right). \end{aligned}$$

*Proof.* By (E.2) and the triangle inequality we have that

$$\sum_{k=1}^{k_0} \left\| \left( \int_0^1 \mathbf{\Sigma}_X(t, k) dt \right) \left( \int_0^1 \mathbf{\Sigma}_X(t, k) dt \right)^\top \right\|_F \asymp p^{2-2\delta}. \quad (\text{F.7})$$

On the other hand, by Weyl's inequality (Bhatia (1997)) and (12) of Lam et al. (2011) we have that

$$\sup_{t \in [0,1]} \left\| \sum_{k=1}^{k_0} \left( \int_0^1 \mathbf{\Sigma}_X(t, k) dt \right) \left( \int_0^1 \mathbf{\Sigma}_X(t, k) dt \right)^\top \right\|_m \geq \left( \int_0^1 \inf_{t \in (0,1)} \|\mathbf{\Sigma}_X(t, 1) dt\|_m \right)^2. \quad (\text{F.8})$$

By (F.7), (F.8) and the proof of Theorem ?? we have that

$$\lambda_d(\mathbf{\Gamma}) \asymp p^{2-2\delta} \quad (\text{F.9})$$

The corollary follows from Corollary F.1, (F.9) and Theorem 1 of Yu et al. (2015). Details are omitted for the sake of brevity.  $\square$

**Proof of Proposition ??.** *Proof.* It follows from Corollaries F.1 and F.2, and the proof of Proposition ??.  $\square$

**Corollary F.3.** *Assume conditions of Proposition ?? hold, then under null hypothesis there exists an orthonormal basis  $\mathbf{F}_i, 1 \leq i \leq p-d$  of null space of  $\mathbf{\Gamma}$ , such that*

$$\|\|\hat{\mathbf{F}} - \mathbf{F}\|_F\|_{\mathcal{L}^1} = O\left(\frac{p^\delta}{\sqrt{n}}\right), \quad (\text{F.10})$$

where  $\mathbf{F} = (\mathbf{F}_1, \dots, \mathbf{F}_{p-d})$ .

*Proof.* Notice that by Corollary F.2, there exists a set of orthogonal basis  $\mathbf{G} = (\mathbf{G}_1, \dots, \mathbf{G}_{p-d})$  of null space of  $\mathbf{\Gamma}$  together with a  $(p-d) \times (p-d)$  orthonormal matrix  $\hat{\mathbf{O}}_4$  such that

$$\|\hat{\mathbf{F}}\hat{\mathbf{O}}_4 - \mathbf{G}\|_F = O\left(\frac{p^\delta}{\sqrt{n}}\right).$$

Take  $\mathbf{F} = \mathbf{G}\hat{\mathbf{O}}_4^\top$  and the corollary is proved.  $\square$

## 6.1 Proof of Proposition ??

*Proof.* By Proposition ??, it suffices to prove everything on the event  $A_n := \{\hat{d}_n = d\}$ . Define  $\hat{\mathbf{Z}}_i$  in analogue to  $\tilde{\mathbf{Z}}_i$ , with  $\mathbf{F}_i$  replaced by  $\hat{\mathbf{F}}_i$ . Then  $\hat{T}_n = |\frac{\sum_{i=1}^{m_n} \hat{\mathbf{Z}}_i}{\sqrt{m_n}}|_\infty$ . Notice that for  $1 \leq s_1 \leq N_n - 1$ ,  $1 \leq s_2 \leq p-d$ ,  $1 \leq s_3 \leq p$ ,  $1 \leq w \leq k_0$ , the  $(k_0(p-d)ps_1 + (w-1)p(p-d) + (s_2-1)p + s_3)_{th}$  entry of  $\tilde{\mathbf{Z}}_i$  and  $\hat{\mathbf{Z}}_i$  are  $\mathbf{F}_{s_2}^\top \mathbf{X}_{s_1 m_n + i + w, n} X_{s_1 m_n + i, s_3}$  and  $\hat{\mathbf{F}}_{s_2}^\top \mathbf{X}_{s_1 m_n + i + w, n} X_{s_1 m_n + i, s_3}$  respectively where  $X_{i, s_2}$  is the  $(s_2)_{th}$  entry of  $\mathbf{X}_{i, n}$ . Let  $\tilde{Z}_{i, s}$  be the  $s_{th}$  entry of  $\tilde{\mathbf{Z}}_i$ , and  $\hat{Z}_{i, s}$  be the  $s_{th}$  entry of  $\hat{\mathbf{Z}}_i$ . Then on event  $A_n$ ,

$$\begin{aligned} |\hat{T}_n - \tilde{T}_n| &= \max_{1 \leq s_1 \leq N_n - 1, 1 \leq s_3 \leq p, 1 \leq w \leq k_0, 1 \leq s_2 \leq p-d} |(\mathbf{F}_{s_2}^\top - \hat{\mathbf{F}}_{s_2}^\top) \sum_{i=1}^{m_n} \mathbf{X}_{s_1 m_n + i + w, n} X_{s_1 m_n + i, s_3}| / \sqrt{m_n} \\ &\leq \max_{1 \leq s_1 \leq N_n - 1, 1 \leq s_3 \leq p, 1 \leq w \leq k_0, 1 \leq s_2 \leq p-d} \sum_{i=1}^{m_n} |(\mathbf{F}_{s_2}^\top - \hat{\mathbf{F}}_{s_2}^\top) \mathbf{X}_{s_1 m_n + i + w, n} X_{s_1 m_n + i, s_3}| / \sqrt{m_n} \quad (\text{F.11}) \end{aligned}$$

By the triangle inequality, condition (M') and Cauchy inequality, it follows that

$$\begin{aligned} &\max_{1 \leq s_2 \leq p-d} |(\mathbf{F}_{s_2}^\top - \hat{\mathbf{F}}_{s_2}^\top) \sum_{i=1}^{m_n} \mathbf{X}_{s_1 m_n + i + w, n} X_{s_1 m_n + i, s_3}| \\ &= \max_{1 \leq s_2 \leq p-d} \left| \sum_{u=1}^p (F_{s_2, u} - \hat{F}_{s_2, u}) \sum_{i=1}^{m_n} X_{s_1 m_n + i + w, u} X_{s_1 m_n + i, s_3} \right| \\ &\leq \max_{1 \leq s_2 \leq p-d} \sqrt{\sum_{u=1}^p (F_{s_2, u} - \hat{F}_{s_2, u})^2} \sqrt{\sum_{u=1}^p \left( \sum_{i=1}^{m_n} X_{s_1 m_n + i + w, u} X_{s_1 m_n + i, s_3} \right)^2} \\ &\leq \|\hat{\mathbf{F}} - \mathbf{F}\|_F \sum_{u=1}^p \left( \sum_{i=1}^{m_n} X_{s_1 m_n + i + w, u} X_{s_1 m_n + i, s_3} \right)^2^{1/2}. \quad (\text{F.12}) \end{aligned}$$

Moreover, for  $1 \leq s_1 \leq N_n - 1$ ,  $1 \leq s_3 \leq p$ ,  $1 \leq w \leq k_0$ ,

$$\begin{aligned} \left\| \sum_{u=1}^p \left( \sum_{i=1}^{m_n} X_{s_1 m_n + i + w, u} X_{s_1 m_n + i, s_3} \right)^2 \right\|_{\mathcal{L}^l}^{1/2} &= \left\| \sum_{u=1}^p \left( \sum_{i=1}^{m_n} X_{s_1 m_n + i + w, u} X_{s_1 m_n + i, s_3} \right)^2 \right\|_{\mathcal{L}^{l/2}}^{1/2} \\ &\lesssim \sqrt{p} m_n. \end{aligned} \quad (\text{F.13})$$

Using the fact that

$$\begin{aligned} \mathbb{E} \left( \max_{\substack{1 \leq s_1 \leq N_n - 1, \\ 1 \leq s_3 \leq p, \\ 1 \leq w \leq k_0}} \left( \left\| \sum_{u=1}^p \left( \sum_{i=1}^{m_n} X_{s_1 m_n + i + w, u} X_{s_1 m_n + i, s_3} \right)^2 \right\|^{1/2} \right)^l \right) &\leq \\ &\sum_{\substack{1 \leq s_1 \leq N_n - 1, \\ 1 \leq s_3 \leq p, \\ 1 \leq w \leq k_0}} \left\| \left\| \sum_{u=1}^p \left( \sum_{i=1}^{m_n} X_{s_1 m_n + i + w, u} X_{s_1 m_n + i, s_3} \right)^2 \right\|^{1/2} \right\|_{\mathcal{L}^l}^l, \end{aligned} \quad (\text{F.14})$$

we have

$$\left\| \max_{\substack{1 \leq s_1 \leq N_n - 1, \\ 1 \leq s_3 \leq p, \\ 1 \leq w \leq k_0}} \left\| \sum_{u=1}^p \left( \sum_{i=1}^{m_n} X_{s_1 m_n + i + w, u} X_{s_1 m_n + i, s_3} \right)^2 \right\|^{1/2} \right\|_{\mathcal{L}^l} = O((N_n p)^{1/l} \sqrt{p} m_n). \quad (\text{F.15})$$

Now the proposition follows from Proposition ??, (F.11), (F.12) and (F.15), Corollary F.3 and an application of (E.17).  $\square$

In the following proofs, define the  $k_0 N_n (p - d) p$  dimensional vectors  $\tilde{\mathbf{Z}}_i$  via replacing  $\hat{\mathbf{F}}$  in  $\hat{\mathbf{Z}}_i$  of (??) with  $\mathbf{F}$ . Further define

$$\mathbf{S}_{j, w_n} = \sum_{r=j}^{j+w_n-1} \tilde{\mathbf{Z}}_r, \quad \mathbf{S}_{m_n} = \sum_{i=1}^{m_n} \tilde{\mathbf{Z}}_i \quad \text{for } 1 \leq j \leq m_n - w_n + 1. \quad (\text{F.16})$$

Notice that by conditions (S1) and (S3),  $\tilde{\mathbf{Z}}_i$ ,  $1 \leq i \leq m_n$  are mean 0  $N_n (p - d) p$  dimensional vectors.

## 6.2 Proof of Theorem ??.

The key idea of the proof of Theorem ?? is to approximate the test statistic by the maximum of the mean of some centered high-dimensional non-stationary time series. Then we shall apply  $\mathcal{L}^\infty$

Gaussian approximation results in the literature such as those of Zhang and Cheng (2018).

We first show (??). To show (??) we verify the conditions of Corollary 2.2 of Zhang and Cheng (2018). Recall the proof of Proposition ?? that for  $1 \leq s_1 \leq N_n - 1$ ,  $1 \leq s_2 \leq p - d$ ,  $1 \leq s_3 \leq p$ ,  $1 \leq w \leq k_0$ , the  $(k_0(p - d)ps_1 + (w - 1)p(p - d) + (s_2 - 1)p + s_3)_{th}$  entry of  $\tilde{\mathbf{Z}}_i$  is  $\mathbf{F}_{s_2}^\top \mathbf{X}_{s_1 m_n + i + w, n} X_{s_1 m_n + i, s_3}$  where  $X_{i, s_2}$  is the  $(s_2)_{th}$  entry of  $\mathbf{X}_{i, n}$ . Let  $\tilde{Z}_{i, s}$  be the  $s_{th}$  entry of  $\tilde{\mathbf{Z}}_i$ . By the proof of Lemma E.3, condition M', condition (a) and the definition of  $\mathbf{X}_{i, n}$ , using the fact that  $\|\mathbf{F}_i\|_F = 1$  for  $1 \leq i \leq p - d$ , we get

$$\delta_{\tilde{\mathbf{Z}}}(j, k, l) := \max_{1 \leq i \leq m_n} \max_{1 \leq s \leq N_n k_0 (p - d)p} \mathbb{E}^{1/l}(|\tilde{Z}_{i, s} - \tilde{Z}_{i, s}^{(i-k)}|^l) = O(((k + 1) \log(k + 1))^{-2}). \quad (\text{F.17})$$

Notice that (F.17) satisfies (10) of Assumption 2.3 of Zhang and Cheng (2018). Furthermore, by the triangle inequality, condition (M') and Cauchy inequality, under null hypothesis, we have

$$\|\mathbf{F}_{s_2}^\top \mathbf{X}_{s_1 m_n + i + w, n} X_{s_1 m_n + i, s_3}\|_{\mathcal{L}^l} \leq \|\mathbf{F}_{s_2}^\top \mathbf{e}_{s_1 m_n + i + w}\|_{\mathcal{L}^{2l}} \|X_{s_1 m_n + i, s_3}\|_{\mathcal{L}^{2l}}.$$

By triangle inequality and condition (M'), we have  $\|X_{s_1 m_n + i, s_3}\|_{\mathcal{L}^{2l}}$  is bounded for  $s_1$ ,  $i$  and  $s_3$ . By conditions (f) we have that

$$\|\mathbf{F}_{s_2}^\top \mathbf{e}_{s_1 m_n + i + w}\|_{\mathcal{L}^{2l}} \leq M_{2l} \|\mathbf{F}_{s_2}^\top \mathbf{e}_{s_1 m_n + i + w}\|_{\mathcal{L}^2}, \quad (\text{F.18})$$

$$\|\mathbf{F}_{s_2}^\top \mathbf{e}_{s_1 m_n + i + w}\|_{\mathcal{L}^2}^2 = \mathbf{F}_{s_2}^\top \mathbb{E}(\mathbf{e}_{s_1 m_n + i + w} \mathbf{e}_{s_1 m_n + i + w}^\top) \mathbf{F}_{s_2} \leq \max_{1 \leq i \leq n} \lambda_{\max}(\text{cov}(\mathbf{e}_{i, n} \mathbf{e}_{i, n}^\top)) \lesssim 1, \quad (\text{F.19})$$

where the  $\lesssim$  in (F.19) is uniformly for all  $i, n, p$ , which is due to condition (f). This leads to that

$$\begin{aligned} & \max_{1 \leq i \leq m_n} \mathbb{E}(\max_{1 \leq s \leq N_n k_0 (p - d)p} |\tilde{Z}_{i, s}|^4) \\ &= \max_{1 \leq i \leq m_n} \mathbb{E}(\max_{1 \leq s_1 \leq N_n - 1, 1 \leq s_3 \leq p, 1 \leq w \leq k_0, 1 \leq s_2 \leq p - d} |\mathbf{F}_{s_2}^\top \mathbf{X}_{s_1 m_n + i + w, n} X_{s_1 m_n + i, s_3}|^4) \lesssim (N_n p^2)^{4/l}, \end{aligned} \quad (\text{F.20})$$

which with condition (c) shows that equation (12) of Corollary 2.2 of Zhang and Cheng (2018) holds. Finally, using (F.17), (F.20) and by similar arguments of Lemma E.3 and Lemma 5 of Zhou and Wu (2010), we shall see that  $\max_{1 \leq j \leq k_0 N_n (p - d)p} \sigma_{j, j} \leq M < \infty$  for some constant  $M$ . This verifies (9) of Zhang and Cheng (2018), which proves the first claim of the theorem.

To see the second claim of the theorem, writing  $\delta_0 = g_n^2 \frac{p^\delta \sqrt{m_n}}{\sqrt{n}} \Omega_n$ , where  $g_n$  is a diverging

sequence. Notice that

$$\mathbb{P}(\hat{T}_n \geq t) \leq \mathbb{P}(\tilde{T}_n \geq t - \delta_0) + \mathbb{P}(|\tilde{T}_n - \hat{T}_n| \geq \delta_0), \quad (\text{F.21})$$

$$\begin{aligned} \mathbb{P}(\hat{T}_n \geq t) &\geq \mathbb{P}(\tilde{T}_n \geq t + \delta_0, |\tilde{T}_n - \hat{T}_n| \leq \delta_0) \\ &= \mathbb{P}(\tilde{T}_n \geq t + \delta_0) - \mathbb{P}(\tilde{T}_n \geq t + \delta_0, |\tilde{T}_n - \hat{T}_n| \geq \delta_0) \\ &\geq \mathbb{P}(\tilde{T}_n \geq t + \delta_0) - \mathbb{P}(|\tilde{T}_n - \hat{T}_n| \geq \delta_0). \end{aligned} \quad (\text{F.22})$$

Therefore following the first assertion of Theorem ?? and Proposition ??, we have

$$\begin{aligned} \sup_{t \in \mathbb{R}} |\mathbb{P}(\hat{T}_n \geq t) - \mathbb{P}(|\mathbf{Y}|_\infty \geq t)| &\leq \sup_t |\mathbb{P}(|\mathbf{Y}|_\infty \geq t - \delta_0) - \mathbb{P}(|\mathbf{Y}|_\infty \geq t + \delta_0)| \\ &\quad + O\left(\frac{1}{g_n} + \frac{p^\delta}{\sqrt{n}} \log n + \iota(m_n, k_0 N_n p(p-d), 2l, (N_n p^2)^{1/l})\right). \end{aligned} \quad (\text{F.23})$$

Since  $|\mathbf{Y}|_\infty = \max(\mathbf{Y}, -\mathbf{Y})$ , by Corollary 1 of Chernozhukov et al. (2015), we have that

$$\sup_t |\mathbb{P}(|\mathbf{Y}|_\infty \geq t - \delta_0) - \mathbb{P}(|\mathbf{Y}|_\infty \geq t + \delta_0)| = O(\delta_0 \sqrt{\log(n/\delta_0)}). \quad (\text{F.24})$$

Combining (F.23) and (F.24), and letting  $g_n = (\frac{p^\delta \sqrt{m_n \log n}}{\sqrt{n}} \Omega_n)^{-1/3}$ , the second claim of Theorem ?? follows.  $\square$

### 6.3 Proof of Theorem ??

Define

$$\mathbf{v}_n = \frac{1}{\sqrt{w(m_n - w_n + 1)}} \sum_{j=1}^{m_n - w_n + 1} (\mathbf{S}_{j, w_n} - \frac{w_n}{m_n} \mathbf{S}_{m_n}) R_j. \quad (\text{F.25})$$

We shall show the following two assertions:

$$\sup_{t \in \mathbb{R}} |\mathbb{P}(|\mathbf{Y}|_\infty \leq t) - \mathbb{P}(|\mathbf{v}_n|_\infty \leq t | \mathbf{X}_{i,n}, 1 \leq i \leq n)| = O_p(\Theta_n^{1/3} \log^{2/3}(\frac{W_{n,p}}{\Theta_n})), \quad (\text{F.26})$$

$$\begin{aligned} \sup_{t \in \mathbb{R}} |\mathbb{P}(|\mathbf{v}_n|_\infty \leq t | \mathbf{X}_{i,n}, 1 \leq i \leq n) - \mathbb{P}(|\boldsymbol{\kappa}_n|_\infty \leq t | \mathbf{X}_{i,n}, 1 \leq i \leq n)| \\ = O_p\left(\left(\frac{p^{\delta+1/2} \sqrt{w_n \log n}}{\sqrt{n}} (N_n p)^{1/l}\right)^{l/(l+1)}\right). \end{aligned} \quad (\text{F.27})$$

The theorem then follows from (F.26), (F.27) and Theorem ???. In the remaining proofs, we write conditional on  $\mathbf{X}_{i,n}$ ,  $1 \leq i \leq n$  as conditional on  $\mathbf{X}_{i,n}$  for short if no confusion arises.

Step (i): Proof of (F.26). To show (F.26), we shall show that

$$\left\| \max_{1 \leq u, v \leq k_0 N_n p(p-d)} |\sigma_{u,v}^v - \sigma_{u,v}^Y| \right\|_{\mathcal{L}^{q^*}} = O \left( w_n^{-1} + \sqrt{w_n/m_n} W_{n,p}^{1/q^*} \right), \quad (\text{F.28})$$

where  $\sigma_{u,v}^v$  and  $\sigma_{u,v}^Y$  are the  $(u, v)_{th}$  entry of the covariance matrix of  $\mathbf{v}_n$  given  $\tilde{\mathbf{Z}}_i$  and covariance matrix of  $\mathbf{Y}$ . Notice that (F.28) together with condition (d) implies that there exists a constant  $\eta_0 > 0$  such that

$$\mathbb{P} \left( \max_{1 \leq u, v \leq k_0 N_n p(p-d)} \sigma_{u,v}^v \geq \eta_0 \right) \geq 1 - O \left( \left( w_n^{-1} + \sqrt{w_n/m_n} W_{n,p}^{1/q^*} \right)^{q^*} \right). \quad (\text{F.29})$$

Since by assumption  $w_n^{-1} + \sqrt{w_n/m_n} W_{n,p}^{1/q^*} = o(1)$ , it suffices to consider the conditional Gaussian approximation on the  $\{\mathbf{X}_{i,n}\}$  measurable event  $\{\max_{1 \leq u, v \leq k_0 N_n p(p-d)} \sigma_{u,v}^v \geq \eta_0\}$ . Then by the construction of  $\mathbf{Y}$  and Theorem 2 of Chernozhukov et al. (2015) (we consider the case  $a_p = \sqrt{2 \log p}$  in there), (F.26) will follow.

Now we prove (F.28). Let  $S_{j,w_n,s}$  and  $S_{m_n,s}$  be the  $s_{th}$  element of the vectors  $\mathbf{S}_{j,w_n}$  and  $\mathbf{S}_{m_n}$ , respectively. By our construction, we have

$$\sigma_{u,v}^v = \frac{1}{w_n(m_n - w_n + 1)} \left( \sum_{j=1}^{m_n - w_n + 1} \left( S_{j,w_n,u} - \frac{w_n}{m_n} S_{m_n,u} \right) \left( S_{j,w_n,v} - \frac{w_n}{m_n} S_{m_n,v} \right) \right), \quad \sigma_{u,v}^Y = \mathbb{E} \frac{S_{m_n,u} S_{m_n,v}}{m_n}. \quad (\text{F.30})$$

On one hand, following the proof of Lemma 4 of Zhou (2013) using conditions (i), (ii) and Lemma 5 of Zhou and Wu (2010) we have that

$$\max_{u,v} |\mathbb{E} \sigma_{u,v}^v - \sigma_{u,v}^Y| = O \left( w_n^{-1} + \sqrt{\frac{w_n}{m_n}} \right). \quad (\text{F.31})$$

Now using (i), (ii) and a similar argument to the proof of Lemma 1 of Zhou (2013), Cauchy-Schwarz

inequality and the fact that  $\max_{1 \leq i \leq m_n} |X_i|^{q^*} \leq \sum_{i=1}^{m_n} |X_i|^{q^*}$ , we obtain that

$$\left\| \max_{u,v} \left| \frac{1}{w_n(m_n - w_n + 1)} \sum_{j=1}^{m_n - w_n + 1} (S_{j,w_n,u} S_{j,w_n,v} - \mathbb{E}(S_{j,w_n,u} S_{j,w_n,v})) \right| \right\|_{\mathcal{L}^{q^*}} = O(\sqrt{w_n/m_n} W_{n,p}^{1/q^*}), \quad (\text{F.32})$$

$$\left\| \max_{u,v} \left| \frac{w_n}{m_n^2(m_n - w_n + 1)} \sum_{j=1}^{m_n - w_n + 1} (S_{m_n,u} S_{m_n,v} - \mathbb{E}(S_{m_n,u} S_{m_n,v})) \right| \right\|_{\mathcal{L}^{q^*}} = O(\sqrt{w_n/m_n} W_{n,p}^{1/q^*}) \quad (\text{F.33})$$

$$\left\| \max_{u,v} \left| \frac{1}{m_n(m_n - w_n + 1)} \sum_{j=1}^{m_n - w_n + 1} (S_{j,w_n,u} S_{m_n,v} - \mathbb{E}(S_{j,w_n,u} S_{m_n,v})) \right| \right\|_{\mathcal{L}^{q^*}} = O(\sqrt{w_n/m_n} W_{n,p}^{1/q^*}), \quad (\text{F.34})$$

$$\left\| \max_{u,v} \left| \frac{1}{m_n(m_n - w_n + 1)} \sum_{j=1}^{m_n - w_n + 1} (S_{j,w_n,v} S_{m_n,u} - \mathbb{E}(S_{j,w_n,v} S_{m_n,u})) \right| \right\|_{\mathcal{L}^{q^*}} = O(\sqrt{w_n/m_n} W_{n,p}^{1/q^*}) \quad (\text{F.35})$$

Combining (F.32)-(F.35) we have

$$\left\| \max_{u,v} |\sigma_{u,v}^v - \mathbb{E}\sigma_{u,v}^v| \right\|_{\mathcal{L}^{q^*}} = O(\sqrt{w_n/m_n} W_{n,p}^{1/q^*}). \quad (\text{F.36})$$

Therefore (F.28) follows from (F.31) and (F.36).

Step(ii). We now show (F.27). It suffices to consider on the event  $\{\hat{d}_n = d\}$ . We first show that for  $\epsilon \in (0, \infty)$

$$\mathbb{P}(|\mathbf{v}_n - \boldsymbol{\kappa}_n|_\infty \geq \epsilon | \mathbf{X}_{i,n}) = O_p((\epsilon^{-1} p^{\delta+1/2} \frac{\sqrt{w_n}}{\sqrt{n}} (N_n p)^{1/l})^l). \quad (\text{F.37})$$

After that we then show for  $\epsilon \in (0, \infty)$

$$\sup_{t \in \mathbb{R}} \mathbb{P}(|\mathbf{v}_n - t| \leq \epsilon | \mathbf{X}_{i,n}) = O_p(\epsilon \sqrt{\log(n/\epsilon)}). \quad (\text{F.38})$$

Combining (F.37) and (F.38), and following the argument of (F.21) to (F.23), we have

$$\sup_{t \in \mathbb{R}} |\mathbb{P}(|\mathbf{v}_n|_\infty \leq t | \mathbf{X}_{i,n}, 1 \leq i \leq n) - \mathbb{P}(|\boldsymbol{\kappa}_n|_\infty \leq t | \mathbf{X}_{i,n}, 1 \leq i \leq n)|$$

$$= O_p((\epsilon^{-1} \frac{p^{\delta+1/2} \sqrt{w_n}}{\sqrt{n}} (N_n p)^{1/l})^l + \epsilon \sqrt{\log(n/\epsilon)}). \quad (\text{F.39})$$

Take  $\epsilon = (\frac{p^{\delta+1/2} \sqrt{w_n}}{\sqrt{n}} (N_n p)^{1/l})^{l/(l+1)} \log^{-1/(2l+2)} n$ , (F.27) follows.

To show (F.37) it suffices to prove that

$$\mathbb{E}(|\frac{1}{\sqrt{w_n(m_n - w_n + 1)}} \sum_{j=1}^{m_n - w_n + 1} (\hat{\mathbf{S}}_{j,w_n} - \mathbf{S}_{j,w_n}) R_j|_\infty^l | \mathbf{X}_{i,n})^{1/l} = O(\frac{p^{\delta+1/2} \sqrt{w_n}}{\sqrt{n}} (N_n p)^{1/l}), \quad (\text{F.40})$$

$$\mathbb{E}(|\frac{1}{\sqrt{w_n(m_n - w_n + 1)}} \sum_{j=1}^{m_n - w_n + 1} \frac{w_n}{m_n} (\hat{\mathbf{S}}_{m_n} - \mathbf{S}_{m_n}) R_j|_\infty^l | \mathbf{X}_{i,n})^{1/l} = O(\frac{p^{\delta+1/2} \sqrt{w_n}}{\sqrt{n}} (N_n p)^{1/l}). \quad (\text{F.41})$$

We now show (F.40), and (F.41) follows mutatis mutandis. Define  $\hat{S}_{j,w_n,r}$  and  $S_{j,w_n,r}$  as the  $r$ th component of the  $k_0 N_n(p-d)p$  dimensional vectors  $\hat{\mathbf{S}}_{j,w_n}$  and  $\mathbf{S}_{j,w_n}$ . Using the notation of proof of Theorem ??, it follows that

$$\begin{aligned} & \left| \sum_{j=1}^{m_n - w_n + 1} (\hat{\mathbf{S}}_{j,w_n} - \mathbf{S}_{j,w_n}) R_j \right|_\infty \\ &= \max_{\substack{1 \leq s_1 \leq N_n - 1, \\ 1 \leq s_3 \leq p, \\ 1 \leq w \leq k_0}} \max_{1 \leq s_2 \leq p-d} \left| \sum_{j=1}^{m_n - w_n + 1} \left( \sum_{i=j}^{j+w_n-1} (\hat{\mathbf{F}}_{s_2}^\top - \mathbf{F}_{s_2}^\top) \mathbf{X}_{s_1 m_n + i + w, n} X_{s_1 m_n + i, s_3} \right) R_j \right|. \end{aligned} \quad (\text{F.42})$$

Notice that

$$\begin{aligned} & \max_{1 \leq s_2 \leq p-d} \left| \sum_{j=1}^{m_n - w_n + 1} \left( \sum_{i=j}^{j+w_n-1} (\hat{\mathbf{F}}_{s_2}^\top - \mathbf{F}_{s_2}^\top) \mathbf{X}_{s_1 m_n + i + w, n} X_{s_1 m_n + i, s_3} \right) R_j \right|^2 \\ & \leq \sum_{1 \leq s_2 \leq p-d} \left\| \hat{\mathbf{F}}_{s_2}^\top - \mathbf{F}_{s_2}^\top \right\|_2^2 \left\| \sum_{j=1}^{m_n - w_n + 1} \sum_{i=j}^{j+w_n-1} \mathbf{X}_{s_1 m_n + i + w, n} X_{s_1 m_n + i, s_3} R_j \right\|_2^2 \\ & = \left\| \hat{\mathbf{F}} - \mathbf{F} \right\|_F^2 \left\| \sum_{j=1}^{m_n - w_n + 1} \sum_{i=j}^{j+w_n-1} \mathbf{X}_{s_1 m_n + i + w, n} X_{s_1 m_n + i, s_3} R_j \right\|_2^2. \end{aligned} \quad (\text{F.43})$$

Therefore, by using Corollary F.3, (F.42), (F.43) we have

$$\left| \sum_{j=1}^{m_n - w_n + 1} (\hat{\mathbf{S}}_{j,w_n} - \mathbf{S}_{j,w_n}) R_j \right|_\infty \leq \frac{p^\delta}{\sqrt{n}} \max_{\substack{1 \leq s_1 \leq N_n - 1, \\ 1 \leq s_3 \leq p, \\ 1 \leq w \leq k_0}} \left\| \sum_{j=1}^{m_n - w_n + 1} \sum_{i=j}^{j+w_n-1} \mathbf{X}_{s_1 m_n + i + w, n} X_{s_1 m_n + i, s_3} R_j \right\|_2. \quad (\text{F.44})$$

Notice that, conditional on  $\mathbf{X}_{i,n}$ ,  $\sum_{j=1}^{m_n-w_n+1} \sum_{i=j}^{j+w_n-1} \mathbf{X}_{s_1 m_n+i+w,n} X_{s_1 m_n+i,s_3} R_j$  are  $p$  dimensional Gaussian random vector for  $1 \leq s_1 \leq N_n - 1$ ,  $1 \leq s_3 \leq p$ ,  $1 \leq w \leq k_0$  whose extreme probabilistic behaviour depend on their covariance structure. Therefore we shall study

$$\left\| \sum_{j=1}^{m_n-w_n+1} \sum_{i=j}^{j+w_n-1} \mathbf{X}_{s_1 m_n+i+w,n} X_{s_1 m_n+i,s_3} \right\|_2.$$

For this purpose, for any random variable  $Y$  write  $(\mathbb{E}(|Y|^l | \mathbf{X}_{i,n}))^{1/l} = \|Y\|_{\mathcal{L}^l, \mathbf{X}_{i,n}}$  then

$$\begin{aligned} & \mathbb{E} \left( \max_{\substack{1 \leq s_1 \leq N_n-1, \\ 1 \leq s_3 \leq p, \\ 1 \leq w \leq k_0}} \left( \left\| \sum_{j=1}^{m_n-w_n+1} \sum_{i=j}^{j+w_n-1} \mathbf{X}_{s_1 m_n+i+w,n} X_{s_1 m_n+i,s_3} R_j \right\|_2^2 \right)^{l/2} \middle| \mathbf{X}_{i,n} \right) \\ & \leq \sum_{\substack{1 \leq s_1 \leq N_n-1, \\ 1 \leq s_3 \leq p, \\ 1 \leq w \leq k_0}} \mathbb{E} \left( \left( \sum_{s=1}^p \left( \sum_{j=1}^{m_n-w_n+1} \sum_{i=j}^{j+w_n-1} X_{s_1 m_n+i+w,s} X_{s_1 m_n+i,s_3} R_j \right)^2 \right)^{l/2} \middle| \mathbf{X}_{i,n} \right) \\ & \leq \sum_{\substack{1 \leq s_1 \leq N_n-1, \\ 1 \leq s_3 \leq p, \\ 1 \leq w \leq k_0}} \left( \sum_{s=1}^p \left\| \left( \sum_{j=1}^{m_n-w_n+1} \sum_{i=j}^{j+w_n-1} X_{s_1 m_n+i+w,s} X_{s_1 m_n+i,s_3} R_j \right)^2 \right\|_{\mathcal{L}^{l/2}, \mathbf{X}_{i,n}} \right)^{l/2} \\ & = \sum_{\substack{1 \leq s_1 \leq N_n-1, \\ 1 \leq s_3 \leq p, \\ 1 \leq w \leq k_0}} \left( \sum_{s=1}^p \left\| \left( \sum_{j=1}^{m_n-w_n+1} \sum_{i=j}^{j+w_n-1} X_{s_1 m_n+i+w,s} X_{s_1 m_n+i,s_3} R_j \right)^2 \right\|_{\mathcal{L}^l, \mathbf{X}_{i,n}} \right)^{l/2}. \end{aligned} \quad (\text{F.45})$$

By Burkholder inequality, conditions (M'), (M1) and (M3), we have that

$$\left\| \left\| \left( \sum_{j=1}^{m_n-w_n+1} \sum_{i=j}^{j+w_n-1} X_{s_1 m_n+i+w,s} X_{s_1 m_n+i,s_3} R_j \right)^2 \right\|_{\mathcal{L}^l, \mathbf{X}_{i,n}} \right\|_{\mathcal{L}^l} \lesssim w_n \sqrt{m_n - w_n + 1}. \quad (\text{F.46})$$

Therefore by straightforward calculations and equations (F.44)–(F.46), we show (F.40). Therefore (F.27) follows.

Finally (F.38) follows from by Corollary 1 of Chernozhukov et al. (2015) and (F.29), which completes the proof.  $\square$

## 7 Proof of Theorem C.1

Recall the quantities  $\check{\mathbf{Z}}_i$  and  $\tilde{\mathbf{Z}}_i$  defined in Section 3, and  $\hat{\mathbf{Z}}_i$  in (??) in the main article. To prove the power result in Theorem C.1 we need to evaluate the magnitude of  $\mathbb{E}\hat{\mathbf{Z}}_i$  under the local alternatives, which are determined by  $\mathbb{E}\tilde{\mathbf{Z}}_i$  and  $\mathbb{E}\check{\mathbf{Z}}_i$ . Define  $\mathbf{X}_i^* = \mathbf{A}\mathbf{z}_{i,n} + \mathbf{e}_{i,n}$ , and further define  $\tilde{\mathbf{Z}}_i^*$  by replacing  $\mathbf{X}_{i,n}$  in  $\tilde{\mathbf{Z}}_i$  with  $\mathbf{X}_{i,n}^*$ . Notice that, under the considered alternative,  $\mathbf{Y}_i$  in fact preserves the autocovariance structure of  $\tilde{\mathbf{Z}}_i^*$ . Then we prove Theorem C.1 by the similar arguments to the proof of Theorems ?? and ?? but under local alternatives.

**Proposition G.1.** *Write  $\Gamma(0)$  as  $\Gamma$ . Under conditions of Theorem C.1, we have that for each  $n$  there exists an orthogonal basis  $\mathbf{F} = (\mathbf{F}_1, \dots, \mathbf{F}_{p-d})$  such that*

$$\|\mathbf{F}_n - \mathbf{F}\|_F = O(\rho_n p^{(\delta-\delta_1)/2}), \quad (\text{G.1})$$

where  $\mathbf{F}$  forms a basis of  $\Gamma$ . Furthermore,

$$\| \|\hat{\mathbf{F}} - \mathbf{F}_n\|_F \|_{\mathcal{L}^1} = O\left(\frac{p^\delta}{\sqrt{n}}\right), \quad \| \|\hat{\mathbf{F}} - \mathbf{F}\|_F \|_{\mathcal{L}^1} = O\left(\rho_n p^{(\delta-\delta_1)/2} + \frac{p^\delta}{\sqrt{n}}\right). \quad (\text{G.2})$$

*Proof.* By the definition of  $\Gamma$  and  $\Gamma_n$ , it follows that  $\|\Gamma_n - \Gamma\| = O(\rho_n p^{\frac{1-\delta_1}{2}} p^{\frac{3(1-\delta)}{2}})$ . Therefore by the proof of Corollaries F.2 and F.3, for each  $n$  there exists an orthogonal basis  $\mathbf{F} = (\mathbf{F}_1, \dots, \mathbf{F}_{p-d})$  such that

$$\|\mathbf{F}_n - \mathbf{F}\|_F = O\left(\frac{\|\Gamma_n - \Gamma\|_F}{p^{2-2\delta}}\right) = O(\rho_n p^{(\delta-\delta_1)/2}), \quad (\text{G.3})$$

which shows (G.1). By the similar argument to Corollary F.1 and triangle inequality, we have that

$$\| \|\hat{\mathbf{F}} - \Gamma_n\|_F \|_{\mathcal{L}^1} = O\left(\frac{p^\delta}{\sqrt{n}} p^{2-2\delta}\right), \quad (\text{G.4})$$

$$\| \|\hat{\mathbf{F}} - \Gamma\|_F \|_{\mathcal{L}^1} \leq \| \|\hat{\mathbf{F}} - \Gamma_n\|_F \|_{\mathcal{L}^1} + \| \|\Gamma_n - \Gamma\|_F \|_{\mathcal{L}^1} = O\left(\left(\rho_n p^{(\delta-\delta_1)/2} + \frac{p^\delta}{\sqrt{n}}\right) p^{2-2\delta}\right), \quad (\text{G.5})$$

which further by Theorem 1 of Yu et al. (2015) yield that

$$\| \|\hat{\mathbf{F}} - \mathbf{F}_n\|_F \|_{\mathcal{L}^1} = O\left(\frac{\| \|\hat{\mathbf{F}} - \Gamma_n\|_F \|_{\mathcal{L}^1}}{p^{2-2\delta}}\right) = O\left(\frac{p^\delta}{\sqrt{n}}\right), \quad (\text{G.6})$$

$$\|\|\hat{\mathbf{F}} - \mathbf{F}\|_F\|_{\mathcal{L}^1} = O\left(\frac{\|\|\hat{\mathbf{\Gamma}} - \mathbf{\Gamma}\|_F\|_{\mathcal{L}^1}}{p^{2-2\delta}}\right) = O(\rho_n p^{(\delta-\delta_1)/2} + \frac{p^\delta}{\sqrt{n}}). \quad (\text{G.7})$$

Therefore (G.2) holds.  $\square$

The following proposition studies the bias of the expectation of  $\check{\mathbf{Z}}_i$  and  $\tilde{\mathbf{Z}}_i$ .

**Proposition G.2.** *Under conditions of Theorem C.1, we have that*

$$|\mathbb{E}\tilde{\mathbf{Z}}_i|_\infty = O(\rho_n p^{\frac{1-\delta_1}{2}}), \quad |\mathbb{E}\check{\mathbf{Z}}_i|_\infty = O(\rho_n p^{\frac{1-\delta_1}{2}}). \quad (\text{G.8})$$

*Proof.* To show the first equation of (G.8), notice that for  $1 \leq s_1 \leq N_n - 1$ ,  $1 \leq s_2 \leq p - d$ ,  $1 \leq s_3 \leq p$ ,  $1 \leq w \leq k_0$ , the  $(k_0(p-d)ps_1 + (w-1)p(p-d) + (s_2-1)p + s_3)_{th}$  entry of  $\mathbb{E}\tilde{\mathbf{Z}}_i$  is  $\mathbb{E}(\mathbf{F}_{s_2}^\top \mathbf{X}_{s_1 m_n + i + w, n} X_{s_1 m_n + i, s_3})$  where  $X_{i, s_2}$  is the  $(s_2)_{th}$  entry of  $\mathbf{X}_{i, n}$ . Then by Cauchy-Schwarz inequality we have that there exists a constant  $M$  such that uniformly for  $1 \leq s_1 \leq N_n - 1$ ,  $1 \leq s_2 \leq p - d$ ,  $1 \leq s_3 \leq p$ ,  $1 \leq w \leq k_0$ ,

$$\begin{aligned} & |\mathbb{E}(\mathbf{F}_{s_2}^\top \mathbf{X}_{s_1 m_n + i + w, n} X_{s_1 m_n + i, s_3})| \\ &= |\mathbb{E}(\mathbf{F}_{s_2}^\top (\rho_n \mathbf{D}(t_n) \circ \mathbf{A} \mathbf{z}_{s_1 m_n + i + w, n} + \mathbf{e}_{s_1 m_n + i + w, n}) X_{s_1 m_n + i, s_3})| \leq \rho_n M p^{\frac{1-\delta_1}{2}}, \end{aligned} \quad (\text{G.9})$$

where  $t_n = (s_1 m_n + i + w)/n$ .

In the above argument we have used the fact that  $\|\mathbf{F}_u\|_F = 1$  for  $1 \leq u \leq p - d$ . Therefore the first equation of (G.8) follows from (G.9). Write  $\mathbf{h}_{s_2} = \mathbf{F}_{s_2} - \mathbf{F}_{s_2, n}$ . Similarly,

$$\begin{aligned} & |\mathbb{E}(\mathbf{h}_{s_2}^\top \mathbf{X}_{s_1 m_n + i + w, n} X_{s_1 m_n + i, s_3})| \\ &= |\mathbb{E}(\mathbf{h}_{s_2}^\top (\mathbf{A}(t_n) \mathbf{z}_{s_1 m_n + i + w, n} + \mathbf{e}_{s_1 m_n + i + w, n}) X_{s_1 m_n + i, s_3})| \\ &\leq |\mathbb{E}(\mathbf{h}_{s_2}^\top (\mathbf{A}(t_n) \mathbf{z}_{s_1 m_n + i + w, n})| + |\mathbb{E}(\mathbf{h}_{s_2}^\top \mathbf{e}_{s_1 m_n + i + w, n} X_{s_1 m_n + i, s_3})| \\ &= O(\rho_n M p^{\frac{1-\delta_1}{2}}), \end{aligned}$$

where the last equality is due to (G.1), condition (C1), condition (f), Cauchy inequality and the submultiplicity of Frobenius norm. Therefore we have  $|\mathbb{E}\check{\mathbf{Z}}_i - \mathbb{E}\tilde{\mathbf{Z}}_i|_\infty = O(\rho_n p^{\frac{1-\delta_1}{2}})$ . Together with first equation of (G.8) we get

$$|\mathbb{E}\check{\mathbf{Z}}_i|_\infty = O(\rho_n p^{\frac{1-\delta_1}{2}}), \quad (\text{G.10})$$

and the proof is complete.  $\square$

**Proof of Theorem C.1.** We first show (a). Now a careful inspection of the proof of Proposition ?? shows that the proposition ?? still holds under considered alternative hypothesis used in Theorem ?. Recall  $\hat{T} = \left| \frac{\sum_{i=1}^{m_n} \hat{\mathbf{Z}}_i}{\sqrt{m_n}} \right|_\infty$ . Define  $\hat{\mathbf{Z}}_i$  in analogue of  $\tilde{\mathbf{Z}}_i$  with  $\mathbf{F}$  replaced by  $\hat{\mathbf{F}}$ . Define

$$\tilde{T}_n = \left| \frac{\sum_{i=1}^{m_n} \tilde{\mathbf{Z}}_i}{\sqrt{m_n}} \right|_\infty, \quad \tilde{T}_n^* = \left| \frac{\sum_{i=1}^{m_n} \tilde{\mathbf{Z}}_i^*}{\sqrt{m_n}} \right|_\infty.$$

Using Proposition G.1 and following the proof of Proposition ?? we have that for any sequence  $g_n \rightarrow \infty$ ,

$$\mathbb{P}(|\tilde{T}_n - \hat{T}_n| \geq g_n^2(\rho_n p^{(\delta-\delta_1)/2} + \frac{p^\delta}{\sqrt{n}})m_n^{1/2}\Omega_n) = O(\frac{1}{g_n} + \frac{p^\delta}{\sqrt{n}} \log n). \quad (\text{G.11})$$

One the other hand, similarly to the proof of Proposition ??, on the event of  $\{\hat{d}_n = d\}$ ,

$$\begin{aligned} |\tilde{T}_n - \tilde{T}_n^*| &\leq \max_{\substack{1 \leq s_1 \leq N_n-1, \\ 1 \leq s_3 \leq p, \\ 1 \leq w \leq k_0, 1 \leq s_2 \leq p-d}} \sum_{i=1}^{m_n} |\mathbf{F}_{s_2}^\top (\mathbf{X}_{s_1 m_n + i + w, n} X_{s_1 m_n + i, s_3} - \mathbf{X}_{s_1 m_n + i + w, n}^* X_{s_1 m_n + i, s_3}^*)| / \sqrt{m_n} \\ &\leq \max_{\substack{1 \leq s_1 \leq N_n-1, \\ 1 \leq s_3 \leq p, \\ 1 \leq w \leq k_0}} \left| \sum_{u=1}^p \left( \sum_{i=1}^{m_n} (X_{s_1 m_n + i + w, u} X_{s_1 m_n + i, s_3} - X_{s_1 m_n + i + w, u}^* X_{s_1 m_n + i, s_3}^*) \right)^2 \right|^{1/2}. \end{aligned} \quad (\text{G.12})$$

Notice that

$$\begin{aligned} &\left\| \sum_{u=1}^p \left( \sum_{i=1}^{m_n} (X_{s_1 m_n + i + w, u} X_{s_1 m_n + i, s_3} - X_{s_1 m_n + i + w, u}^* X_{s_1 m_n + i, s_3}^*) \right)^2 \right\|_{\mathcal{L}^t}^{1/2} \\ &= \left\| \sum_{u=1}^p \left( \sum_{i=1}^{m_n} X_{s_1 m_n + i + w, u} X_{s_1 m_n + i, s_3} - X_{s_1 m_n + i + w, u}^* X_{s_1 m_n + i, s_3}^* \right)^2 \right\|_{\mathcal{L}^t}^{1/2} \end{aligned} \quad (\text{G.13})$$

which can be further bounded by the summation of

$$\left\| 2 \sum_{u=1}^p \left( \sum_{i=1}^{m_n} X_{s_1 m_n + i + w, u} (X_{s_1 m_n + i, s_3} - X_{s_1 m_n + i, s_3}^*) \right)^2 \right\|_{\mathcal{L}^t}^{1/2}$$

and

$$\left\| 2 \sum_{u=1}^p \left( \sum_{i=1}^{m_n} X_{s_1 m_n + i, s_3}^* (X_{s_1 m_n + i + w, u} - X_{s_1 m_n + i + w, u}^*) \right)^2 \right\|_{\mathcal{L}^{l/2}}^{1/2}.$$

Therefore, using the definition of  $\mathbf{X}_{i,n}^*$  straightforward calculations show that

$$\left\| \sum_{u=1}^p \left( \sum_{i=1}^{m_n} (X_{s_1 m_n + i + w, u} X_{s_1 m_n + i, s_3} - X_{s_1 m_n + i + w, u}^* X_{s_1 m_n + i, s_3}^*) \right)^2 \right\|_{\mathcal{L}^l}^{1/2} \lesssim \sqrt{p} m_n \rho_n. \quad (\text{G.14})$$

As a consequence, by the proof of Proposition ??, for any sequence  $g_n \rightarrow \infty$ ,

$$\mathbb{P}(|\tilde{T}_n^* - \tilde{T}_n| \geq g_n \rho_n m_n^{1/2} \Omega_n) = O\left(\frac{1}{g_n} + \frac{p^\delta}{\sqrt{n}} \log n\right). \quad (\text{G.15})$$

Notice that  $\mathbf{Y}_i$  preserves the autocovariance structure of  $\tilde{\mathbf{Z}}_i^*$ . Then it follows from (G.11), (G.14) and the proof of Theorem ?? that under the alternative hypothesis,

$$\begin{aligned} & \sup_{t \in \mathbb{R}} |\mathbb{P}(\hat{T}_n \leq t) - \mathbb{P}(|\mathbf{Y}|_\infty \leq t)| \\ &= O\left( \left( \left( \rho_n p^{\frac{\delta-\delta_1}{2}} + \frac{p^\delta}{\sqrt{n}} \right) \sqrt{m_n \log n \Omega_n} \right)^{1/3} + \left( \rho_n \sqrt{m_n \log n \Omega_n} \right)^{1/2} + \iota(m_n, k_0 N_n p(p-d), 2l, (N_n p^2)^{1/l}) \right), \end{aligned} \quad (\text{G.16})$$

which proves (C.7). We now show the divergence case in (a).

Define  $\check{\mathbf{T}} = \frac{\sum_{i=1}^{m_n} \check{\mathbf{Z}}_i}{\sqrt{m_n}}$  and notice that  $\hat{\mathbf{T}} = \frac{\sum_{i=1}^{m_n} \hat{\mathbf{Z}}_i}{\sqrt{m_n}}$ . Following the proof of Proposition ?? we have that

$$|\check{\mathbf{T}} - \hat{\mathbf{T}}|_\infty = O_p\left(\frac{p^\delta}{\sqrt{n}} m_n^{1/2} \Omega_n\right). \quad (\text{G.17})$$

Notice that for  $1 \leq s_1 \leq N_n - 1$ ,  $1 \leq s_2 \leq p - d$ ,  $1 \leq s_3 \leq p$ ,  $1 \leq w \leq k_0$ , the  $(k_0(p-d)ps_1 + (w-1)p(p-d) + (s_2-1)p + s_3)_{th}$  entry of  $\check{\mathbf{Z}}_i$  is  $\mathbf{F}_{s_2, n}^\top \mathbf{X}_{s_1 m_n + i + w, n} X_{s_1 m_n + i, s_3}$  where  $X_{i, s_2}$  is the  $(s_2)_{th}$  entry of  $\mathbf{X}_{i, n}$ . It is easy to see that

$$|\check{\mathbf{T}}|_\infty \geq \frac{1}{\sqrt{m_n}} \left| \sum_{i=1}^{m_n} \mathbf{F}_{s_2, n}^\top \mathbf{X}_{s_1 m_n + i + w, n} X_{s_1 m_n + i, s_3} \right|, \quad (\text{G.18})$$

where by the definition of and the conditions on  $\Delta_n, s_1, s_2, s_3, w$  can be chosen such that

$$\frac{1}{\sqrt{m_n}} \sum_{i=1}^{m_n} \mathbb{E}(\mathbf{F}_{s_2,n}^\top \mathbf{X}_{s_1 m_n + i + w, n} X_{s_1 m_n + i, s_3}) \asymp (\sqrt{m_n} \rho_n p^{\frac{1-\delta_1}{2}}) \quad (\text{G.19})$$

On the other hand, notice that

$$\begin{aligned} & \frac{1}{m_n} \text{Var} \left( \sum_{i=1}^{m_n} (\mathbf{F}_{s_2,n}^\top \mathbf{X}_{s_1 m_n + i + w, n} X_{s_1 m_n + i, s_3}) \right) \\ &= \frac{1}{m_n} \sum_{i_1, i_2} \text{Cov}(\mathbf{F}_{s_2,n}^\top \mathbf{X}_{s_1 m_n + i_1 + w, n} X_{s_1 m_n + i_1, s_3}, \mathbf{F}_{s_2,n}^\top \mathbf{X}_{s_1 m_n + i_2 + w, n} X_{s_1 m_n + i_2, s_3}). \end{aligned} \quad (\text{G.20})$$

Consider the case when  $i_1 > i_2$ . Now using condition (G) and that

$$\mathbf{X}_{s_1 m_n + i_1 + w, n} = \mathbf{A} \left( \frac{s_1 m_n + i_1 + w, n}{n} \right) \mathbf{z}_{s_1 m_n + i_1 + w, n} + e_{s_1 m_n + i_1 + w, n},$$

we have (let  $i'_1 = s_1 m_n + i_1, i'_2 = s_1 m_n + i_2$  for short)

$$\begin{aligned} \text{Cov}(\mathbf{F}_{s_2,n}^\top \mathbf{X}_{i'_1 + w, s_3}, \mathbf{F}_{s_2,n}^\top \mathbf{X}_{i'_2 + w, s_3}) &= \text{Cov}(\mathbf{F}_{s_2,n}^\top \mathbf{A} \left( \frac{i'_2 + w}{n} \right) \mathbf{z}_{i'_1 + w, s_3}, \mathbf{F}_{s_2,n}^\top \mathbf{A} \left( \frac{i'_2 + w}{n} \right) \mathbf{z}_{i'_2 + w, s_3}) \\ &\quad + \text{Cov}(\mathbf{F}_{s_2,n}^\top \mathbf{A} \left( \frac{i'_2 + w}{n} \right) \mathbf{z}_{i'_1 + w, s_3}, \mathbf{F}_{s_2,n}^\top \mathbf{e}_{i'_2 + w, s_3}). \end{aligned} \quad (\text{G.21})$$

Notice that (G.1) and condition (C1) lead to

$$\|\mathbf{F}_{s_2,n}^\top \mathbf{A} \left( \frac{k}{n} \right)\|_F = O(\rho_n p^{\frac{1-\delta_1}{2}}) \quad (\text{G.22})$$

uniformly for  $1 \leq s_2 \leq p - d$  and  $1 \leq k \leq n$ . Therefore,

$$\begin{aligned} & \text{Cov}(\mathbf{F}_{s_2,n}^\top \mathbf{A} \left( \frac{i'_2 + w}{n} \right) \mathbf{z}_{i'_1 + w, s_3}, \mathbf{F}_{s_2,n}^\top \mathbf{A} \left( \frac{i'_2 + w}{n} \right) \mathbf{z}_{i'_2 + w, s_3}) \\ &= \|\mathbf{F}_{s_2,n}^\top \mathbf{A} \left( \frac{i'_2 + w}{n} \right) \text{Cov}(\mathbf{z}_{i'_1 + w, s_3}, \mathbf{z}_{i'_2 + w, s_3}) (\mathbf{F}_{s_2,n}^\top \mathbf{A} \left( \frac{i'_2 + w}{n} \right))^\top\|_F \\ &\leq \rho_n^2 p^{1-\delta_1} \|\text{Cov}(\mathbf{z}_{i'_1 + w, s_3}, \mathbf{z}_{i'_2 + w, s_3})\|_F. \end{aligned} \quad (\text{G.23})$$

On the other hand using condition (G2) and condition (ii) of Theorem ??, by the proof of Lemma E.3 it follows for  $1 \leq u \leq d, \leq v \leq p, \Upsilon_{i,u,v} =: \Upsilon_{i,u,v}(\frac{i}{n}, \mathcal{F}_i) = z_{i,u,n} x_{i+k,v,n}$  is a locally stationary

process with associated dependence measures

$$\delta_{\mathbf{r}_{u,v},2}(h) = O(((k+1)\log(k+1))^{-2}). \quad (\text{G.24})$$

Therefore by Lemma 5 of Zhou and Wu (2010), uniformly for  $1 \leq i_1, i'_2 \leq m_n$  and  $1 \leq s_3 \leq p$ ,

$$\|Cov(\mathbf{z}_{i'_1+w}X_{i'_1,s_3}, \mathbf{z}_{i'_2+w}X_{i'_2,s_3})\|_F = O((|i'_2 - i'_1| \log(|i'_2 - i'_1|))^{-2}). \quad (\text{G.25})$$

Together with (G.23) we have

$$\frac{1}{m_n} \sum_{i'_1, i'_2} Cov(\mathbf{F}_{s_2,n}^\top \mathbf{A}(\frac{i'_2+w}{n}) \mathbf{z}_{i'_1+w}X_{i'_1}, \mathbf{F}_{s_2,n}^\top \mathbf{A}(\frac{i'_2+w}{n}) \mathbf{z}_{i'_2+w}X_{i'_2}) = O(\rho_n^2 p^{1-\delta_1} \vee 1). \quad (\text{G.26})$$

By similarly arguments using the proof of Lemma 5 of Zhou and Wu (2010) and condition (G3) we have

$$\frac{1}{m_n} \sum_{i'_1, i'_2} Cov(\mathbf{F}_{s_2,n}^\top \mathbf{A}(\frac{i'_2+w}{n}) \mathbf{z}_{i'_1+w}X_{i'_1}, \mathbf{F}_{s_2,n}^\top \mathbf{e}_{i'_2+w}X_{i'_2}) = O(\rho_n p^{\frac{1-\delta_1}{2}} \log^2 p \vee 1) \quad (\text{G.27})$$

By (G.18)–(G.20), (G.26) and (G.27) we show  $\hat{T}_n$  is diverging at the rate of  $\sqrt{m}\rho_n p^{\frac{1-\delta_1}{2}}$ , which proves (a).

To show (b), we define

$$\mathbf{S}_{j,w_n}^* = \sum_{r=j}^{j+w_n-1} \tilde{\mathbf{Z}}_r^*, \quad \mathbf{S}_{m_n}^* = \sum_{i=1}^{m_n} \tilde{\mathbf{Z}}_i^* \quad \text{for } 1 \leq j \leq m_n - w_n + 1. \quad (\text{G.28})$$

Then we define

$$\mathbf{v}_n^* = \frac{1}{\sqrt{w_n(m_n - w_n + 1)}} \sum_{j=1}^{m_n - w_n + 1} (\mathbf{S}_{j,w_n}^* - \frac{w_n}{m_n} \mathbf{S}_{m_n}^*) R_j, \quad (\text{G.29})$$

$$\tilde{\mathbf{\kappa}}_n = \frac{1}{\sqrt{w_n(m_n - w_n + 1)}} \sum_{j=1}^{m_n - w_n + 1} (\tilde{\mathbf{S}}_{j,w_n} - \frac{w_n}{m_n} \tilde{\mathbf{S}}_{m_n}) R_j. \quad (\text{G.30})$$

Then by the proof of Theorem ?? we have that

$$\sup_{t \in \mathbb{R}} |\mathbb{P}(|\mathbf{Y}|_\infty \leq t) - \mathbb{P}(|\mathbf{v}_n^*|_\infty \leq t | \mathbf{X}_{i,n}, 1 \leq i \leq n)| = O_p(\Theta_n^{1/3} \log^{2/3}(\frac{W_{n,p}}{\Theta_n})). \quad (\text{G.31})$$

Straightforward calculations using similar arguments to the proofs of step (ii) of Theorem ?? and equation (G.2) further show that under the considered local alternative hypothesis,

$$\| |\mathbf{v}_n^* - \tilde{\boldsymbol{\kappa}}_n|_\infty \|_{\mathcal{L}^l, \mathbf{X}_{i,n}} \|_{\mathcal{L}^l} = O(\rho_n \sqrt{w_n} \Omega_n), \quad (\text{G.32})$$

$$\| |\boldsymbol{\kappa}_n - \tilde{\boldsymbol{\kappa}}_n|_\infty \|_{\mathcal{L}^l, \mathbf{X}_{i,n}} \|_{\mathcal{L}^l} = O((\frac{p^\delta}{\sqrt{n}} + \rho_n p^{\frac{\delta-\delta_1}{2}}) \sqrt{w_n} \Omega_n), \quad (\text{G.33})$$

Therefore

$$\| |\mathbf{v}_n^* - \boldsymbol{\kappa}_n|_\infty \|_{\mathcal{L}^l, \mathbf{X}_{i,n}} \|_{\mathcal{L}^l} = O((\frac{p^\delta}{\sqrt{n}} + \rho_n) \sqrt{w_n} \Omega_n). \quad (\text{G.34})$$

As a result, by the arguments of (F.39), (C.8) follows.

To evaluate  $\boldsymbol{\kappa}_n$ , notice that  $\boldsymbol{\kappa}_n$  is a Gaussian vector conditional on  $\{\mathbf{X}_{i,n}\}$ . Therefore

$$\mathbb{E}(|\boldsymbol{\kappa}_n|_\infty | (\mathbf{X}_{i,n})_{1 \leq i \leq n}) \leq |(\sum_{j=1}^{m_n-w_n+1} (\hat{\mathbf{S}}_{j,w_n} - \frac{w_n}{m_n} \hat{\mathbf{S}}_n)^{\circ 2})^{\circ \frac{1}{2}}|_\infty \sqrt{2 \log n / \sqrt{w_n(m_n - w_n + 1)}}, \quad a.s.. \quad (\text{G.35})$$

In the following we consider the event  $\{\hat{d}_n = d\}$ . Observe that

$$|(\sum_{j=1}^{m_n-w_n+1} (\hat{\mathbf{S}}_{j,w_n} - \frac{w_n}{m_n} \hat{\mathbf{S}}_n)^{\circ 2})^{\circ \frac{1}{2}}|_\infty \leq M_1 |(\sum_{j=1}^{m_n-w_n+1} (\hat{\mathbf{S}}_{j,w_n} - \check{\mathbf{S}}_{j,w_n} - \frac{w_n}{m_n} (\hat{\mathbf{S}}_n - \check{\mathbf{S}}_n))^{\circ 2})^{\circ \frac{1}{2}}|_\infty \quad (\text{G.36})$$

$$+ M_1 |(\sum_{j=1}^{m_n-w_n+1} (\check{\mathbf{S}}_{j,w_n} - \mathbb{E} \check{\mathbf{S}}_{j,w_n} - \frac{w_n}{m_n} (\check{\mathbf{S}}_n - \mathbb{E} \check{\mathbf{S}}_n))^{\circ 2})^{\circ \frac{1}{2}}|_\infty + M_1 |(\sum_{j=1}^{m_n-w_n+1} (\mathbb{E} \check{\mathbf{S}}_{j,w_n} - \frac{w_n}{m_n} \mathbb{E} \check{\mathbf{S}}_n)^{\circ 2})^{\circ \frac{1}{2}}|_\infty \\ := I + II + III$$

for some large positive constant  $M_1$ , where  $I$ ,  $II$  and  $III$  are defined in an obvious way.

For  $I$ , notice that similar to the proof of Theorem ?? and the first equality of (G.1), we have

$$I/\sqrt{w_n(m_n - w_n + 1)} = O_p\left(\frac{p^\delta}{\sqrt{n}}\sqrt{w_n\Omega_n}\right). \quad (\text{G.37})$$

For  $II$ , by (G.26), (G.27) and a similar argument to the proof of Theorem ?? applied to  $\check{\mathbf{S}}_{j,w_n}$  and  $\check{\mathbf{S}}_n$ , we shall see that

$$II/\sqrt{w_n(m_n - w_n + 1)} = O_p(\rho_n p^{\frac{1-\delta_1}{2}} \log^2 p \vee \rho_n^2 p^{1-\delta_1} \vee 1). \quad (\text{G.38})$$

For  $III$ , by Proposition G.2

$$III/\sqrt{w_n(m_n - w_n + 1)} = O(\sqrt{w_n}\rho_n p^{\frac{1-\delta_1}{2}}). \quad (\text{G.39})$$

Therefore from (G.35) to (G.39),  $|\boldsymbol{\kappa}_n|_\infty = O_p(\sqrt{w_n}\rho_n p^{\frac{1-\delta_1}{2}}\sqrt{\log n})$ , which completes the proof.  $\square$

## References

- Bhatia, R. (1982). Analysis of spectral variation and some inequalities. *Transactions of the American Mathematical Society*, 272(1):323–331.
- Bhatia, R. (1997). *Matrix analysis*. Springer-Verlag.
- Chen, X. (2007). Large sample sieve estimation of semi-nonparametric models. *Handbook of econometrics*, 6:5549–5632.
- Chernozhukov, V., Chetverikov, D., and Kato, K. (2015). Comparison and anti-concentration bounds for maxima of gaussian random vectors. *Probability Theory and Related Fields*, 162(1):47–70.
- Hansen, B. E. (2014). Nonparametric sieve regression: Least squares, averaging least squares, and cross-validation. *Handbook of Applied Nonparametric and Semiparametric Econometrics and Statistics*, forthcoming.
- Lam, C. and Yao, Q. (2012). Factor modeling for high-dimensional time series: inference for the number of factors. *The Annals of Statistics*, 40(2):694–726.

- Lam, C., Yao, Q., and Bathia, N. (2011). Estimation of latent factors for high-dimensional time series. *Biometrika*, 98(4):901–918.
- Wang, H. and Xiang, S. (2012). On the convergence rates of legendre approximation. *Mathematics of Computation*, 81(278):861–877.
- Yu, Y., Wang, T., and Samworth, R. J. (2015). A useful variant of the davis–kahan theorem for statisticians. *Biometrika*, 102(2):315–323.
- Zhang, X. and Cheng, G. (2018). Gaussian approximation for high dimensional vector under physical dependence. *Bernoulli*, 24(4A):2640–2675.
- Zhou, Z. (2013). Heteroscedasticity and autocorrelation robust structural change detection. *Journal of the American Statistical Association*, 108(502):726–740.
- Zhou, Z. and Wu, W. B. (2009). Local linear quantile estimation for nonstationary time series. *The Annals of Statistics*, 37(5B):2696–2729.
- Zhou, Z. and Wu, W. B. (2010). Simultaneous inference of linear models with time varying coefficients. *Journal of the Royal Statistical Society: Series B (Statistical Methodology)*, 72(4):513–531.
